# Supplementary material for: The search for alternating surgeries
Source: arXiv:2409.09842 ancillary file (2026-05-07)
Supplement: Supplementary file 1 [file data.pdf]

**ADDITIONAL DATA FOR THE ARTICLE 'THE SEARCH FOR  
ALTERNATING SURGERIES'**

KENNETH L. BAKER, MARC KEGEL, AND DUNCAN MCCOY

TABLE 1. The census  
knots in  $\mathcal{D}$ .

| Knot        | $\rho(K)$               | $N$ |
|-------------|-------------------------|-----|
| $t01834$    | $[7, 7, 5, 2]$          | 130 |
| $o9\_03412$ | $[11, 7, 4, 4]$         | 206 |
| $t04003$    | $[7, 7, 4, 2]$          | 120 |
| $v0570$     | $[5, 5, 5, 3]$          | 87  |
| $o9\_15633$ | $[12, 7, 4, 3, 2]$      | 224 |
| $o9\_08852$ | $[14, 8, 6, 3, 3]$      | 317 |
| $t09455$    | $[7, 7, 3, 3, 3]$       | 128 |
| $t04382$    | $[10, 6, 3, 3]$         | 157 |
| $o9\_26791$ | $[11, 6, 3, 2]$         | 172 |
| $o9\_08042$ | $[7, 7, 7, 4, 3, 3]$    | 184 |
| $v1832$     | $[6, 5, 3, 3]$          | 82  |
| $t00855$    | $[8, 8, 5, 3]$          | 165 |
| $o9\_35549$ | $[11, 11, 5, 5, 3, 2]$  | 307 |
| $o9\_13182$ | $[6, 6, 6, 5, 2, 2, 2]$ | 147 |
| $t05663$    | $[8, 7, 4, 3]$          | 141 |
| $v1628$     | $[7, 4, 3, 3]$          | 86  |
| $v2215$     | $[5, 5, 4, 3, 2]$       | 81  |
| $t10681$    | $[11, 5, 5, 3, 2]$      | 186 |
| $o9\_02350$ | $[10, 10, 7, 3, 3, 2]$  | 273 |
| $o9\_08765$ | $[7, 7, 7, 4, 2]$       | 169 |
| $o9\_05357$ | $[11, 8, 3, 3, 2, 2]$   | 213 |
| $o9\_13508$ | $[13, 6, 4, 3]$         | 233 |
| $o9\_16157$ | $[9, 9, 9, 5, 3, 2]$    | 283 |
| $v0740$     | $[4, 4, 4, 4, 3, 2]$    | 79  |
| $o9\_12144$ | $[10, 9, 3, 3, 3]$      | 211 |
| $o9\_11248$ | $[11, 4, 4, 4]$         | 173 |
| $o9\_35736$ | $[11, 11, 6, 3, 3]$     | 299 |
| $o9\_27155$ | $[11, 5, 3, 2]$         | 161 |
| $t01424$    | $[9, 9, 5, 4, 2, 2]$    | 213 |
| $t03979$    | $[8, 6, 3, 2]$          | 115 |
| $o9\_03932$ | $[9, 5, 5]$             | 136 |
| $o9\_23955$ | $[7, 7, 7, 4]$          | 167 |
| $v0082$     | $[5, 5, 5, 2]$          | 82  |
| $o9\_02772$ | $[9, 2, 2, 2]$          | 96  |
| $t10643$    | $[6, 6, 6, 5, 3, 2]$    | 148 |
| $v0847$     | $[7, 4, 4]$             | 85  |
| $o9\_16748$ | $[7, 7, 7, 5, 3, 2]$    | 187 |
| $o9\_39394$ | $[8, 7, 4, 2, 2]$       | 139 |
| $t09016$    | $[9, 5, 4, 3, 2]$       | 137 |
| $o9\_05860$ | $[10, 10, 3, 3, 3, 2]$  | 233 |
| $v0223$     | $[7, 7, 4, 3, 2]$       | 129 |
| $o9\_27261$ | $[8, 8, 7, 3, 3, 2]$    | 201 |
| $o9\_28113$ | $[6, 6, 6, 6, 5, 3, 2]$ | 184 |

| Knot        | $\rho(K)$               | $N$ |
|-------------|-------------------------|-----|
| $t01216$    | $[10, 4, 3, 3]$         | 137 |
| $o9\_03526$ | $[6, 5, 5]$             | 91  |
| $o9\_35772$ | $[6, 6, 4, 3, 3]$       | 109 |
| $s407$      | $[7, 4, 2, 2]$          | 75  |
| $t02639$    | $[11, 7, 4, 3, 2]$      | 201 |
| $o9\_05229$ | $[12, 5, 5, 2]$         | 201 |
| $o9\_03032$ | $[9, 7, 2, 2, 2, 2]$    | 148 |
| $v2024$     | $[6, 6, 5, 2, 2]$       | 107 |
| $o9\_14364$ | $[7, 7, 6, 2, 2]$       | 144 |
| $o9\_24149$ | $[7, 7, 7, 3, 3, 3]$    | 177 |
| $o9\_08647$ | $[14, 5, 5, 4, 2, 2]$   | 272 |
| $o9\_04313$ | $[13, 6, 5, 2, 2]$      | 240 |
| $o9\_12919$ | $[11, 5, 4, 2]$         | 168 |
| $v1839$     | $[9, 5, 3, 2]$          | 121 |
| $t05674$    | $[6, 6, 6, 5, 2, 2]$    | 143 |
| $v1966$     | $[8, 6, 3, 3]$          | 121 |
| $v0497$     | $[8, 5, 3, 3]$          | 110 |
| $o9\_14495$ | $[10, 7, 3, 3, 2, 2]$   | 177 |
| $o9\_23023$ | $[9, 9, 5, 4, 3, 2]$    | 218 |
| $o9\_13400$ | $[8, 8, 7, 2, 2, 2]$    | 191 |
| $t01598$    | $[11, 5, 4, 2, 2]$      | 172 |
| $t09852$    | $[6, 5, 3]$             | 73  |
| $o9\_05970$ | $[13, 8, 5, 3]$         | 270 |
| $t10985$    | $[11, 6, 3, 3]$         | 178 |
| $t04019$    | $[5, 5, 4, 4]$          | 86  |
| $t01636$    | $[11, 4, 4, 3, 2]$      | 168 |
| $o9\_13188$ | $[6, 6, 6, 6, 4, 3]$    | 172 |
| $v0573$     | $[5, 5, 5, 2, 2, 2]$    | 89  |
| $o9\_13056$ | $[11, 8, 4, 4]$         | 221 |
| $o9\_23263$ | $[11, 4, 4, 3, 3]$      | 174 |
| $o9\_35320$ | $[6, 6, 5, 4, 2]$       | 119 |
| $o9\_23977$ | $[9, 8, 3, 3, 3]$       | 175 |
| $o9\_13125$ | $[10, 7, 4, 3]$         | 177 |
| $o9\_24886$ | $[14, 6, 6, 3, 3]$      | 289 |
| $v1300$     | $[7, 3]$                | 62  |
| $t01318$    | $[9, 4, 3, 2, 2]$       | 116 |
| $o9\_13952$ | $[13, 5, 5, 2, 2]$      | 229 |
| $v0330$     | $[7, 2, 2]$             | 60  |
| $o9\_06248$ | $[11, 11, 4, 4, 2, 2]$  | 284 |
| $o9\_08776$ | $[14, 6, 5, 3, 2]$      | 272 |
| $t06440$    | $[8, 8, 3, 3, 3]$       | 158 |
| $o9\_03586$ | $[7, 7, 7, 2, 2, 2, 2]$ | 165 |
| $o9\_14376$ | $[10, 10, 6, 3, 3]$     | 257 |
| $o9\_01680$ | $[8, 8, 8, 3, 2, 2]$    | 211 |
| $o9\_12757$ | $[5, 5, 5, 5, 5, 3, 3]$ | 146 |
| $v1921$     | $[8, 5, 2, 2]$          | 99  |

ADDITIONAL DATA FOR THE ARTICLE 'THE SEARCH FOR ALTERNATING SURGERIES'3

| Knot            | $\rho(K)$             | $N$ | Knot            | $\rho(K)$                | $N$ |
|-----------------|-----------------------|-----|-----------------|--------------------------|-----|
| <i>t08111</i>   | [5, 5, 3, 3, 2]       | 74  | <i>o9_13537</i> | [11, 6, 5, 2, 2, 2]      | 196 |
| <i>o9_28746</i> | [11, 5, 5, 3, 3]      | 192 | <i>o9_11999</i> | [13, 7, 5, 2, 2]         | 253 |
| <i>o9_11570</i> | [11, 3, 3, 3, 3]      | 160 | <i>t05578</i>   | [9, 8, 3, 3, 2]          | 169 |
| <i>o9_06154</i> | [9, 9, 5, 3, 2, 2]    | 206 | <i>v1718</i>    | [8, 3, 3, 3]             | 94  |
| <i>t02238</i>   | [8, 8, 3, 3]          | 149 | <i>v1620</i>    | [4, 4, 4, 3, 3]          | 69  |
| <i>v1547</i>    | [7, 4, 2]             | 71  | <i>o9_34403</i> | [8, 6, 3]                | 112 |
| <i>t00434</i>   | [7, 7, 7, 4, 3, 2]    | 178 | <i>t02404</i>   | [9, 5, 3, 2, 2]          | 125 |
| <i>t05538</i>   | [5, 5, 5, 4, 3, 2]    | 106 | <i>o9_18007</i> | [7, 7, 6, 4, 3]          | 162 |
| <i>m144</i>     | [3, 3, 3, 2, 2]       | 37  | <i>o9_30790</i> | [13, 6, 6, 3, 3]         | 262 |
| <i>v2090</i>    | [9, 4, 4, 2, 2]       | 123 | <i>o9_08006</i> | [11, 8, 3, 3, 3]         | 215 |
| <i>o9_02655</i> | [9, 9, 4, 3, 2, 2]    | 197 | <i>t02378</i>   | [11, 4, 4, 2, 2]         | 163 |
| <i>m276</i>     | [5, 4, 2, 2]          | 51  | <i>o9_32257</i> | [7, 6, 3]                | 97  |
| <i>o9_15997</i> | [13, 9, 4, 3, 2]      | 281 | <i>v0939</i>    | [5, 5, 4, 2]             | 72  |
| <i>o9_11560</i> | [11, 11, 6, 5, 3, 2]  | 318 | <i>t03864</i>   | [7, 7, 4, 3, 2, 2]       | 133 |
| <i>o9_02386</i> | [10, 10, 6, 4, 3]     | 264 | <i>o9_22663</i> | [9, 5, 5, 2, 2]          | 141 |
| <i>t04102</i>   | [7, 7, 3, 3, 2, 2]    | 126 | <i>s344</i>     | [6, 4, 3]                | 64  |
| <i>t05425</i>   | [6, 6, 5, 3, 3]       | 118 | <i>t02398</i>   | [8, 8, 5, 3, 2, 2]       | 172 |
| <i>o9_12693</i> | [5, 5, 5, 4, 4]       | 111 | <i>t00324</i>   | [3, 3, 3, 3, 3, 3, 2, 2] | 64  |
| <i>o9_29436</i> | [9, 9, 8, 3, 3, 2]    | 250 | <i>t03956</i>   | [7, 6, 2, 2]             | 95  |
| <i>o9_01953</i> | [5, 5, 5, 5, 5, 3]    | 137 | <i>o9_30375</i> | [11, 6, 5, 3, 3]         | 203 |
| <i>t06463</i>   | [9, 9, 5, 3, 2]       | 202 | <i>o9_23961</i> | [10, 7, 3, 3, 3]         | 179 |
| <i>o9_28529</i> | [13, 7, 4, 3]         | 246 | <i>o9_28153</i> | [9, 9, 5, 2, 2]          | 197 |
| <i>o9_14079</i> | [13, 4, 4, 4, 2, 2]   | 227 | <i>o9_01955</i> | [5, 5, 5, 5, 5, 2, 2, 2] | 139 |
| <i>v0114</i>    | [5, 5, 5, 3, 2, 2]    | 94  | <i>o9_24592</i> | [8, 5, 2]                | 96  |
| <i>v0407</i>    | [8, 3, 3, 2, 2]       | 92  | <i>m270</i>     | [5, 3, 3]                | 46  |
| <i>o9_16181</i> | [13, 8, 5, 3, 3]      | 279 | <i>o9_04269</i> | [5, 5, 5, 5, 4, 2]       | 122 |
| <i>o9_15506</i> | [11, 7, 4, 3, 2, 2]   | 205 | <i>s582</i>     | [4, 4, 3, 3]             | 53  |
| <i>m071</i>     | [5, 2]                | 32  | <i>o9_28810</i> | [9, 9, 4, 4, 3, 2]       | 209 |
| <i>t00932</i>   | [8, 8, 5, 3, 3]       | 174 | <i>o9_02786</i> | [4, 4, 4, 4, 4, 3, 2, 2] | 99  |
| <i>o9_09808</i> | [13, 9, 4, 4, 2, 2]   | 292 | <i>t05564</i>   | [6, 6, 6, 4, 3]          | 136 |
| <i>v0434</i>    | [8, 5, 3]             | 101 | <i>m240</i>     | [4, 3, 3]                | 37  |
| <i>t03607</i>   | [10, 4, 4, 3]         | 144 | <i>o9_18633</i> | [11, 5, 5, 2, 2, 2]      | 185 |
| <i>t01949</i>   | [8, 7, 2, 2, 2]       | 127 | <i>t06570</i>   | [8, 8, 5, 2, 2]          | 163 |
| <i>s104</i>     | [7, 3, 2, 2]          | 68  | <i>t00873</i>   | [8, 8, 3, 2, 2]          | 147 |
| <i>s800</i>     | [5, 5, 3, 3]          | 71  | <i>t05239</i>   | [11, 5, 3, 3]            | 167 |
| <i>v1392</i>    | [7, 3, 2]             | 64  | <i>o9_35682</i> | [6, 6, 5, 3]             | 109 |
| <i>t08403</i>   | [9, 4, 2, 2]          | 107 | <i>t03709</i>   | [7, 7, 4, 3, 3]          | 135 |
| <i>o9_24889</i> | [9, 9, 7, 3, 3]       | 232 | <i>o9_01584</i> | [8, 8, 8, 3, 3, 2, 2]    | 220 |
| <i>o9_05426</i> | [7, 7, 7, 7, 3, 3, 2] | 220 | <i>s294</i>     | [5, 4, 2]                | 47  |
| <i>o9_05618</i> | [12, 7, 5, 2, 2, 2]   | 232 | <i>v1980</i>    | [5, 3, 3, 2]             | 49  |
| <i>o9_18209</i> | [7, 7, 7, 4, 4]       | 183 | <i>o9_13666</i> | [11, 7, 3, 3]            | 191 |
| <i>o9_04431</i> | [13, 7, 6, 2, 2, 2]   | 268 | <i>o9_14831</i> | [8, 3, 2]                | 80  |
| <i>s086</i>     | [3, 3, 3, 3, 2, 2]    | 46  | <i>o9_05483</i> | [7, 7, 7, 7, 4, 2, 2]    | 222 |
| <i>o9_16065</i> | [14, 9, 5, 4, 2, 2]   | 328 | <i>o9_00168</i> | [5, 5, 5, 5, 5, 3, 2, 2] | 144 |
| <i>o9_22477</i> | [8, 3, 3, 3, 2]       | 97  | <i>v1716</i>    | [7, 3, 3, 2, 2]          | 77  |
| <i>t05426</i>   | [11, 6, 5, 3, 2]      | 197 | <i>t01037</i>   | [5, 5, 5, 5, 2, 2, 2]    | 114 |

| Knot            | $\rho(K)$             | $N$ | Knot            | $\rho(K)$                | $N$ |
|-----------------|-----------------------|-----|-----------------|--------------------------|-----|
| <i>t05658</i>   | [7, 6, 4, 3]          | 113 | <i>t04721</i>   | [7, 7, 6, 2, 2, 2]       | 148 |
| <i>t01292</i>   | [10, 6, 4, 3]         | 164 | <i>s665</i>     | [5, 5, 4, 2, 2]          | 76  |
| <i>o9_22925</i> | [6, 6, 5, 4, 2, 2]    | 123 | <i>o9_14716</i> | [7, 7, 7, 6, 2, 2, 2]    | 197 |
| <i>s369</i>     | [6, 5, 2, 2]          | 71  | <i>t08267</i>   | [8, 7, 3, 3, 2]          | 137 |
| <i>s068</i>     | [5, 5, 3, 2, 2]       | 69  | <i>o9_03108</i> | [9, 2, 2, 2, 2, 2]       | 103 |
| <i>m016</i>     | [3, 2, 2]             | 19  | <i>o9_05562</i> | [13, 5, 5, 3, 2, 2]      | 238 |
| <i>t11852</i>   | [6, 5, 3, 3, 2]       | 85  | <i>o9_11845</i> | [8, 7, 2, 2, 2, 2]       | 131 |
| <i>m082</i>     | [3, 3, 2, 2]          | 28  | <i>t09704</i>   | [8, 8, 6, 3, 3]          | 185 |
| <i>o9_07945</i> | [12, 7, 5, 3, 2]      | 233 | <i>t00423</i>   | [7, 7, 7, 3, 2, 2]       | 166 |
| <i>o9_24183</i> | [14, 8, 5, 3, 2]      | 300 | <i>t01690</i>   | [11, 7, 4, 2, 2]         | 196 |
| <i>v1690</i>    | [7, 4, 3, 2, 2]       | 84  | <i>o9_02255</i> | [10, 10, 3, 3, 2, 2]     | 228 |
| <i>o9_02735</i> | [9, 9, 9, 5, 4, 2, 2] | 294 | <i>o9_04106</i> | [12, 5, 5, 2, 2, 2]      | 208 |
| <i>o9_19130</i> | [7, 6, 5, 2, 2]       | 120 | <i>t02537</i>   | [7, 7, 7, 3, 3, 2]       | 171 |
| <i>o9_21918</i> | [5, 5, 5, 3, 3, 2]    | 99  | <i>t01125</i>   | [10, 3, 3, 2, 2]         | 128 |
| <i>t01646</i>   | [11, 6, 5, 2, 2]      | 192 | <i>m194</i>     | [5, 3]                   | 37  |
| <i>t00729</i>   | [7, 7, 2, 2]          | 109 | <i>o9_04245</i> | [13, 5, 5, 3]            | 231 |
| <i>o9_33526</i> | [7, 4, 4, 2, 2]       | 91  | <i>o9_23660</i> | [11, 7, 4]               | 190 |
| <i>v3354</i>    | [6, 6, 5, 3, 2]       | 112 | <i>t10230</i>   | [6, 4, 3, 3]             | 73  |
| <i>o9_27480</i> | [11, 4, 4]            | 157 | <i>t02567</i>   | [7, 7, 7, 4, 2, 2]       | 173 |
| <i>o9_08224</i> | [7, 7, 7, 3, 2]       | 162 | <i>t01033</i>   | [5, 5, 5, 5, 3]          | 112 |
| <i>v0398</i>    | [7, 5, 2, 2, 2]       | 88  | <i>o9_02706</i> | [9, 9, 9, 4, 3, 2]       | 274 |
| <i>o9_08828</i> | [13, 5, 5, 3, 3]      | 240 | <i>o9_12736</i> | [9, 8, 4, 4]             | 181 |
| <i>o9_22698</i> | [9, 9, 4, 2, 2]       | 188 | <i>v1728</i>    | [6, 5, 2, 2, 2]          | 75  |
| <i>o9_08477</i> | [4, 4, 4, 4, 4, 3, 3] | 101 | <i>o9_16920</i> | [8, 5, 3, 3, 2]          | 113 |
| <i>v2759</i>    | [7, 4]                | 69  | <i>o9_24534</i> | [9, 4, 4, 4]             | 133 |
| <i>o9_16642</i> | [11, 11, 6, 4, 2, 2]  | 304 | <i>o9_25595</i> | [10, 3, 3, 3, 3]         | 139 |
| <i>v1077</i>    | [7, 7, 3, 3, 2]       | 122 | <i>t03713</i>   | [7, 7, 3, 2]             | 113 |
| <i>o9_03802</i> | [11, 3, 3, 3]         | 151 | <i>t04180</i>   | [5, 5, 5, 5, 4, 2, 2]    | 126 |
| <i>t01757</i>   | [7, 7, 2, 2, 2, 2]    | 116 | <i>o9_03162</i> | [11, 11, 4, 4, 3, 2]     | 289 |
| <i>o9_03133</i> | [11, 3, 3, 3, 2, 2]   | 158 | <i>s346</i>     | [7, 3, 3, 2]             | 73  |
| <i>o9_13403</i> | [11, 7, 4, 2]         | 192 | <i>v0945</i>    | [8, 5, 3, 2, 2]          | 108 |
| <i>t00826</i>   | [8, 8, 3, 3, 2, 2]    | 156 | <i>o9_09213</i> | [5, 5, 5, 5, 5, 4, 2, 2] | 151 |
| <i>t02470</i>   | [10, 7, 3, 2, 2]      | 168 | <i>o9_02696</i> | [9, 9, 5, 4, 2]          | 209 |
| <i>t03566</i>   | [7, 7, 3]             | 111 | <i>o9_12412</i> | [10, 7, 3, 2]            | 164 |
| <i>t09313</i>   | [7, 7, 6, 3, 3]       | 155 | <i>o9_04435</i> | [9, 8, 2, 2, 2, 2]       | 163 |
| <i>t02104</i>   | [9, 4, 4, 2]          | 119 | <i>o9_13720</i> | [10, 10, 4, 4, 3]        | 244 |
| <i>o9_27392</i> | [7, 7, 7, 6, 3, 3]    | 204 | <i>m103</i>     | [5, 3, 2, 2]             | 44  |
| <i>o9_03313</i> | [11, 8, 3, 3]         | 206 | <i>v0165</i>    | [3, 3, 3, 3, 3, 2, 2]    | 55  |
| <i>t06001</i>   | [7, 7, 4, 4]          | 134 | <i>o9_06301</i> | [11, 11, 7, 4, 3, 2]     | 322 |
| <i>o9_14018</i> | [13, 7, 6, 3, 3]      | 275 | <i>o9_05021</i> | [8, 8, 8, 3, 3]          | 213 |
| <i>m118</i>     | [4, 3, 2]             | 31  | <i>v1940</i>    | [7, 6, 3, 3]             | 106 |
| <i>o9_17450</i> | [11, 6, 4, 2]         | 179 | <i>o9_22607</i> | [9, 5]                   | 111 |
| <i>o9_10696</i> | [9, 4]                | 102 | <i>o9_01436</i> | [7, 7, 7, 2, 2]          | 158 |
| <i>o9_13639</i> | [8, 8, 6, 3, 2]       | 179 | <i>v1709</i>    | [7, 5, 3, 2]             | 89  |
| <i>t04228</i>   | [9, 7, 3, 3]          | 151 | <i>t03781</i>   | [4, 4, 4, 4, 3, 3]       | 85  |
| <i>o9_16356</i> | [8, 8, 8, 3, 3, 3]    | 222 | <i>o9_14974</i> | [11, 8, 3, 2, 2]         | 204 |

ADDITIONAL DATA FOR THE ARTICLE 'THE SEARCH FOR ALTERNATING SURGERIES'<sup>5</sup>

| Knot            | $\rho(K)$                | $N$ | Knot            | $\rho(K)$             | $N$ |
|-----------------|--------------------------|-----|-----------------|-----------------------|-----|
| <i>o9_29246</i> | [8, 8, 8, 6, 3, 3]       | 249 | <i>t10462</i>   | [9, 4, 4, 3, 2]       | 128 |
| <i>o9_08875</i> | [13, 8, 5, 2, 2]         | 268 | <i>s042</i>     | [5, 5, 2]             | 57  |
| <i>o9_12971</i> | [6, 6, 6, 5, 3, 3]       | 154 | <i>v0759</i>    | [8, 3, 3]             | 85  |
| <i>o9_12873</i> | [14, 5, 5, 3, 2]         | 261 | <i>v1986</i>    | [6, 6, 4, 3]          | 100 |
| <i>t08201</i>   | [7, 4, 4, 2]             | 87  | <i>o9_02340</i> | [10, 10, 4, 3, 3]     | 237 |
| <i>o9_14136</i> | [9, 5, 4, 4]             | 142 | <i>o9_37941</i> | [6, 6, 5, 3, 3, 2]    | 121 |
| <i>t07348</i>   | [6, 5, 4, 2, 2]          | 87  | <i>o9_00815</i> | [7, 7, 7, 7, 4, 3, 2] | 227 |
| <i>o9_33585</i> | [8, 6, 3, 3, 2]          | 124 | <i>t05390</i>   | [6, 6, 5, 2, 2, 2]    | 111 |
| <i>o9_20219</i> | [10, 8, 3, 3, 2]         | 188 | <i>s336</i>     | [4, 4, 3, 2, 2]       | 51  |
| <i>t01850</i>   | [8, 5, 4]                | 109 | <i>v2930</i>    | [7, 3, 3, 3]          | 79  |
| <i>o9_08302</i> | [7, 7, 7, 4, 3, 2, 2]    | 182 | <i>o9_18813</i> | [9, 6, 4, 2]          | 139 |
| <i>v0220</i>    | [7, 7, 3, 2, 2]          | 117 | <i>o9_00133</i> | [5, 5, 5, 5, 5, 2]    | 132 |
| <i>t00787</i>   | [7, 7, 5, 2, 2, 2]       | 137 | <i>t01368</i>   | [9, 5, 4, 2]          | 128 |
| <i>m281</i>     | [4, 4, 3, 2]             | 47  | <i>o9_11685</i> | [10, 3, 3, 3, 2, 2]   | 137 |
| <i>o9_14599</i> | [13, 6, 6, 2, 2, 2]      | 255 | <i>t09267</i>   | [7, 7, 4]             | 118 |
| <i>o9_03833</i> | [9, 7, 2, 2]             | 141 | <i>o9_26604</i> | [9, 6, 4, 2, 2]       | 143 |
| <i>t00110</i>   | [5, 5, 5, 5, 2]          | 107 | <i>o9_16319</i> | [9, 9, 9, 4, 4, 2, 2] | 285 |
| <i>t09954</i>   | [6, 5, 4, 2]             | 83  | <i>s684</i>     | [5, 4, 3, 2]          | 56  |
| <i>t01440</i>   | [4, 4, 4, 4, 4, 3, 2]    | 95  | <i>t06605</i>   | [9, 9, 4, 4, 2, 2]    | 204 |
| <i>t00146</i>   | [5, 5, 5, 5, 3, 2, 2]    | 119 | <i>o9_04205</i> | [12, 7, 5, 2]         | 225 |
| <i>m198</i>     | [5, 2, 2, 2]             | 39  | <i>o9_29529</i> | [8, 7, 5, 3, 2]       | 153 |
| <i>s367</i>     | [4, 4, 4, 3, 2]          | 63  | <i>t01268</i>   | [10, 7, 3, 3, 2]      | 173 |
| <i>v0741</i>    | [9, 5, 4, 2, 2]          | 132 | <i>o9_22129</i> | [10, 3, 3]            | 122 |
| <i>o9_06060</i> | [9, 9, 4, 4, 2]          | 200 | <i>o9_16141</i> | [11, 11, 5, 5, 2, 2]  | 302 |
| <i>o9_27737</i> | [10, 7, 3]               | 162 | <i>o9_13649</i> | [11, 4, 4, 2]         | 159 |
| <i>o9_12519</i> | [5, 5, 5, 5, 4, 3, 2]    | 131 | <i>v1810</i>    | [5, 5, 5, 4, 2, 2]    | 101 |
| <i>o9_30721</i> | [7, 7, 4, 4, 2]          | 136 | <i>o9_00797</i> | [7, 7, 7, 7, 3, 2, 2] | 215 |
| <i>o9_03149</i> | [11, 11, 6, 5, 2, 2]     | 313 | <i>o9_13052</i> | [8, 8, 5, 4]          | 173 |
| <i>o9_03188</i> | [11, 11, 7, 4, 2, 2]     | 317 | <i>t01863</i>   | [10, 3, 3, 3, 2]      | 133 |
| <i>s769</i>     | [6, 5, 3, 2]             | 76  | <i>o9_06128</i> | [10, 10, 7, 3, 2, 2]  | 268 |
| <i>o9_05177</i> | [8, 8, 8, 5, 3, 2, 2]    | 236 | <i>o9_07893</i> | [12, 5, 4, 3, 2]      | 200 |
| <i>o9_13433</i> | [12, 5, 5, 3, 2]         | 209 | <i>v0715</i>    | [9, 4, 3, 2]          | 112 |
| <i>o9_02794</i> | [4, 4, 4, 4, 4, 4, 3, 2] | 111 | <i>o9_01765</i> | [8, 8, 8, 5, 3, 3]    | 238 |
| <i>m239</i>     | [4, 3, 2, 2]             | 35  | <i>o9_03288</i> | [11, 4, 3, 3]         | 158 |
| <i>v2325</i>    | [5, 5, 5, 3, 3]          | 96  | <i>t02099</i>   | [5, 5, 5, 4, 2]       | 97  |
| <i>o9_03118</i> | [11, 11, 5, 4, 2, 2]     | 293 | <i>o9_11467</i> | [11, 11, 5, 3, 3]     | 288 |
| <i>o9_16527</i> | [8, 8, 8, 5, 2, 2]       | 227 | <i>s308</i>     | [5, 5, 2, 2, 2]       | 64  |
| <i>o9_07943</i> | [7, 7, 7, 3]             | 160 | <i>v0709</i>    | [5, 4, 4]             | 61  |
| <i>t06525</i>   | [7, 7, 5, 3, 2]          | 138 | <i>o9_08771</i> | [14, 9, 5, 3, 2]      | 317 |
| <i>t09580</i>   | [9, 5, 2, 2]             | 116 | <i>v0424</i>    | [8, 3, 2, 2]          | 83  |
| <i>v0554</i>    | [7, 2, 2, 2, 2]          | 67  | <i>o9_31165</i> | [11, 7, 4, 3, 3]      | 207 |
| <i>o9_01496</i> | [7, 7, 7, 5, 2, 2, 2]    | 186 | <i>o9_12459</i> | [8, 7, 4, 4]          | 149 |
| <i>o9_07790</i> | [11, 3, 3, 2, 2]         | 149 | <i>o9_12892</i> | [11, 4, 4, 3, 2, 2]   | 172 |
| <i>t01422</i>   | [4, 4, 4, 4, 3, 2, 2]    | 83  | <i>o9_21893</i> | [7, 4, 4, 3]          | 93  |
| <i>o9_09465</i> | [13, 4, 4, 3, 2]         | 216 | <i>o9_13604</i> | [6, 6, 6, 6, 5, 2, 2] | 179 |
| <i>o9_12230</i> | [11, 9, 3, 3, 3]         | 232 | <i>o9_08831</i> | [7, 7, 7, 3, 3, 2, 2] | 175 |

| Knot             | $\rho(K)$                | $N$ |
|------------------|--------------------------|-----|
| <i>v</i> 0765    | [7, 5, 2]                | 81  |
| <i>o</i> 9_04438 | [13, 8, 5, 3, 2, 2]      | 277 |
| <i>o</i> 9_28592 | [8, 8, 7, 4, 3]          | 205 |
| <i>t</i> 05118   | [11, 6, 4, 2, 2]         | 183 |
| <i>s</i> 114     | [7, 4, 3, 2]             | 80  |
| <i>o</i> 9_03622 | [7, 7, 7, 5, 2]          | 179 |
| <i>t</i> 04244   | [11, 5, 5, 2, 2]         | 181 |
| <i>v</i> 0912    | [7, 6, 2, 2, 2]          | 99  |
| <i>o</i> 9_11795 | [10, 3, 3, 2]            | 124 |
| <i>v</i> 1109    | [7, 7, 4, 2, 2]          | 124 |
| <i>o</i> 9_00644 | [3, 3, 3, 3, 3, 3, 2, 2] | 73  |
| <i>v</i> 0707    | [4, 4, 4, 3, 2, 2]       | 67  |
| <i>t</i> 01409   | [9, 9, 4, 3, 2]          | 193 |
| <i>t</i> 05695   | [5, 5, 5, 5, 3, 3]       | 121 |
| <i>o</i> 9_01621 | [8, 8, 8, 5, 3]          | 229 |
| <i>s</i> 301     | [5, 5, 3]                | 62  |

TABLE 2. The hyperbolic integer alternating surgeries

| knot     | slope   | branching set | knot     | slope   | branching set | knot     | slope   | branching set |
|----------|---------|---------------|----------|---------|---------------|----------|---------|---------------|
| v1392    | (-2, 1) | K10a119       | v1547    | (-2, 1) | L10a80        | v1690    | (-2, 1) | L10a106       |
| v1716    | (2, 1)  | K10a98        | v1728    | (2, 1)  | K10a95        | t03713   | (-2, 1) | L11a328       |
| t03864   | (2, 1)  | K11a215       | t03956   | (-2, 1) | L11a377       | t04003   | (-2, 1) | K11a158       |
| t04102   | (2, 1)  | L11a239       | t05390   | (-2, 1) | K11a296       | t09580   | (-1, 1) | K11a148       |
| t10230   | (1, 1)  | K10a97        | t10462   | (-1, 1) | L11a321       | t11556   | (-1, 1) | L9a20         |
| t11852   | (1, 1)  | K10a45        | o9_08224 | (2, 1)  | K12a1178      | o9_08302 | (2, 1)  | L12a1298      |
| o9_08765 | (-2, 1) | L12a987       | o9_08831 | (-2, 1) | K12a977       | o9_11685 | (2, 1)  | K12a1169      |
| o9_11795 | (-2, 1) | K12a952       | o9_11845 | (-2, 1) | K12a1238      | o9_12412 | (2, 1)  | K12a660       |
| o9_12892 | (-2, 1) | L12a998       | o9_12919 | (-2, 1) | K12a1236      | o9_13182 | (-2, 1) | K12a1262      |
| o9_13403 | (-2, 1) | K12a262       | o9_13537 | (-2, 1) | L12a912       | o9_13649 | (2, 1)  | L12a1313      |
| o9_14364 | (-2, 1) | K12a1047      | o9_14495 | (-2, 1) | K12a617       | o9_15506 | (2, 1)  | K12a349       |
| o9_17450 | (-2, 1) | L12a821       | o9_18633 | (-2, 1) | K12a779       | o9_23977 | (1, 1)  | K12a989       |
| o9_26791 | (-1, 1) | K12a321       | o9_27155 | (1, 1)  | L12a923       | o9_27261 | (-1, 1) | K12a635       |
| o9_28153 | (1, 1)  | L12a1133      | o9_28746 | (-1, 1) | L12a1097      | o9_28810 | (1, 1)  | K12a403       |
| o9_30375 | (1, 1)  | K12a284       | o9_32132 | (0, 1)  | K10a45        | o9_32257 | (1, 1)  | L11a313       |
| o9_32588 | (0, 1)  | L10a106       | o9_33526 | (-1, 1) | K10a72        | o9_34403 | (-1, 1) | K11a137       |
| o9_35320 | (0, 1)  | K11a312       | o9_35682 | (1, 1)  | K11a295       | o9_35772 | (-1, 1) | K11a320       |
| o9_37754 | (1, 1)  | L10a76        | o9_37941 | (-1, 1) | K11a115       | o9_39394 | (1, 1)  | K11a217       |
| o9_39451 | (1, 1)  | K10a99        | o9_43001 | (0, 1)  | L10a71        | o9_43679 | (0, 1)  | K11a227       |
| o9_43953 | (0, 1)  | K11a304       | o9_44054 | (0, 1)  | L11a229       |          |         |               |

DEPARTMENT OF MATHEMATICS, UNIVERSITY OF MIAMI, CORAL GABLES, FL 33146, USA  
*Email address:* [k.baker@math.miami.edu](mailto:k.baker@math.miami.edu)

HUMBOLDT-UNIVERSITÄT ZU BERLIN, RUDOWER CHAUSSEE 25, 12489 BERLIN, GERMANY.

RUHR-UNIVERSITÄT BOCHUM, UNIVERSITÄTSSTRASSE 150, 44780 BOCHUM, GERMANY  
*Email address:* [kegemarc@math.hu-berlin.de](mailto:kegemarc@math.hu-berlin.de), [kegemarc87@gmail.com](mailto:kegemarc87@gmail.com)

DÉPARTEMENT DE MATHÉMATIQUES, UNIVERSITÉ DU QUÉBEC À MONTRÉAL, CANADA  
*Email address:* [mc\\_coy.duncan@uqam.ca](mailto:mc_coy.duncan@uqam.ca)

TABLE 3. The lens space surgeries

| knot            | slope   | lens space          | knot            | slope   | lens space          | knot            | slope   | lens space          |
|-----------------|---------|---------------------|-----------------|---------|---------------------|-----------------|---------|---------------------|
| <i>m016</i>     | (-1, 1) | <i>L</i> (19, 7)    | <i>m016</i>     | (0, 1)  | <i>L</i> (18, 5)    | <i>m071</i>     | (-1, 1) | <i>L</i> (31, 11)   |
| <i>m071</i>     | (0, 1)  | <i>L</i> (32, 7)    | <i>m082</i>     | (0, 1)  | <i>L</i> (27, 8)    | <i>m103</i>     | (0, 1)  | <i>L</i> (43, 12)   |
| <i>m118</i>     | (-1, 1) | <i>L</i> (30, 11)   | <i>m118</i>     | (0, 1)  | <i>L</i> (31, 12)   | <i>m144</i>     | (0, 1)  | <i>L</i> (36, 11)   |
| <i>m194</i>     | (0, 1)  | <i>L</i> (37, 10)   | <i>m198</i>     | (1, 1)  | <i>L</i> (39, 16)   | <i>m239</i>     | (0, 1)  | <i>L</i> (34, 13)   |
| <i>m240</i>     | (1, 0)  | <i>L</i> (37, 10)   | <i>m270</i>     | (1, 0)  | <i>L</i> (45, 19)   | <i>m276</i>     | (1, 0)  | <i>L</i> (50, 19)   |
| <i>m281</i>     | (1, 1)  | <i>L</i> (46, 17)   | <i>s042</i>     | (0, 1)  | <i>L</i> (57, 16)   | <i>s068</i>     | (0, 1)  | <i>L</i> (68, 19)   |
| <i>s086</i>     | (0, 1)  | <i>L</i> (45, 14)   | <i>s104</i>     | (-1, 1) | <i>L</i> (68, 19)   | <i>s104</i>     | (0, 1)  | <i>L</i> (67, 18)   |
| <i>s114</i>     | (-1, 1) | <i>L</i> (79, 29)   | <i>s114</i>     | (0, 1)  | <i>L</i> (80, 31)   | <i>s294</i>     | (0, 1)  | <i>L</i> (47, 13)   |
| <i>s336</i>     | (-1, 1) | <i>L</i> (50, 19)   | <i>s344</i>     | (1, 0)  | <i>L</i> (63, 17)   | <i>s346</i>     | (0, 1)  | <i>L</i> (73, 27)   |
| <i>s367</i>     | (1, 1)  | <i>L</i> (62, 23)   | <i>s369</i>     | (1, 0)  | <i>L</i> (71, 21)   | <i>s407</i>     | (0, 1)  | <i>L</i> (75, 29)   |
| <i>s665</i>     | (0, 1)  | <i>L</i> (75, 29)   | <i>s684</i>     | (0, 1)  | <i>L</i> (55, 21)   | <i>s800</i>     | (0, 1)  | <i>L</i> (70, 29)   |
| <i>v0082</i>    | (0, 1)  | <i>L</i> (82, 23)   | <i>v0114</i>    | (0, 1)  | <i>L</i> (93, 25)   | <i>v0165</i>    | (0, 1)  | <i>L</i> (54, 17)   |
| <i>v0220</i>    | (0, 1)  | <i>L</i> (116, 45)  | <i>v0220</i>    | (1, 1)  | <i>L</i> (117, 43)  | <i>v0223</i>    | (0, 1)  | <i>L</i> (129, 49)  |
| <i>v0223</i>    | (1, 1)  | <i>L</i> (128, 47)  | <i>v0330</i>    | (1, 1)  | <i>L</i> (59, 24)   | <i>v0407</i>    | (0, 1)  | <i>L</i> (91, 27)   |
| <i>v0424</i>    | (1, 0)  | <i>L</i> (83, 19)   | <i>v0434</i>    | (0, 1)  | <i>L</i> (101, 30)  | <i>v0497</i>    | (1, 0)  | <i>L</i> (109, 45)  |
| <i>v0554</i>    | (1, 1)  | <i>L</i> (67, 29)   | <i>v0707</i>    | (-1, 1) | <i>L</i> (66, 25)   | <i>v0709</i>    | (1, 0)  | <i>L</i> (61, 13)   |
| <i>v0715</i>    | (1, 0)  | <i>L</i> (112, 31)  | <i>v0740</i>    | (1, 1)  | <i>L</i> (78, 29)   | <i>v0741</i>    | (1, 0)  | <i>L</i> (131, 50)  |
| <i>v0759</i>    | (0, 1)  | <i>L</i> (85, 26)   | <i>v0847</i>    | (1, 0)  | <i>L</i> (84, 25)   | <i>v0912</i>    | (1, 0)  | <i>L</i> (98, 27)   |
| <i>v1300</i>    | (0, 1)  | <i>L</i> (61, 16)   | <i>v1392</i>    | (-1, 1) | <i>L</i> (64, 23)   | <i>v1547</i>    | (-1, 1) | <i>L</i> (77, 27)   |
| <i>v1709</i>    | (0, 1)  | <i>L</i> (89, 34)   | <i>v1810</i>    | (0, 1)  | <i>L</i> (100, 39)  | <i>v1832</i>    | (0, 1)  | <i>L</i> (81, 31)   |
| <i>v1839</i>    | (0, 1)  | <i>L</i> (121, 46)  | <i>v1921</i>    | (0, 1)  | <i>L</i> (99, 29)   | <i>v1980</i>    | (0, 1)  | <i>L</i> (49, 18)   |
| <i>v1986</i>    | (0, 1)  | <i>L</i> (99, 29)   | <i>v2215</i>    | (0, 1)  | <i>L</i> (80, 31)   | <i>v2325</i>    | (0, 1)  | <i>L</i> (95, 39)   |
| <i>v2930</i>    | (0, 1)  | <i>L</i> (79, 23)   | <i>t00110</i>   | (0, 1)  | <i>L</i> (107, 25)  | <i>t00146</i>   | (0, 1)  | <i>L</i> (118, 25)  |
| <i>t00324</i>   | (0, 1)  | <i>L</i> (63, 20)   | <i>t00423</i>   | (-1, 1) | <i>L</i> (166, 49)  | <i>t00423</i>   | (0, 1)  | <i>L</i> (165, 49)  |
| <i>t00434</i>   | (0, 1)  | <i>L</i> (178, 49)  | <i>t00434</i>   | (1, 1)  | <i>L</i> (177, 49)  | <i>t00826</i>   | (0, 1)  | <i>L</i> (155, 46)  |
| <i>t00855</i>   | (0, 1)  | <i>L</i> (165, 49)  | <i>t00873</i>   | (1, 0)  | <i>L</i> (147, 62)  | <i>t00932</i>   | (1, 0)  | <i>L</i> (173, 64)  |
| <i>t01125</i>   | (0, 1)  | <i>L</i> (127, 27)  | <i>t01216</i>   | (1, 0)  | <i>L</i> (137, 37)  | <i>t01268</i>   | (0, 1)  | <i>L</i> (173, 64)  |
| <i>t01292</i>   | (1, 0)  | <i>L</i> (163, 44)  | <i>t01318</i>   | (0, 1)  | <i>L</i> (115, 34)  | <i>t01368</i>   | (0, 1)  | <i>L</i> (128, 47)  |
| <i>t01409</i>   | (1, 0)  | <i>L</i> (193, 81)  | <i>t01422</i>   | (-1, 1) | <i>L</i> (82, 31)   | <i>t01424</i>   | (1, 0)  | <i>L</i> (212, 81)  |
| <i>t01440</i>   | (1, 1)  | <i>L</i> (94, 35)   | <i>t01598</i>   | (1, 0)  | <i>L</i> (171, 50)  | <i>t01636</i>   | (0, 1)  | <i>L</i> (167, 46)  |
| <i>t01646</i>   | (1, 0)  | <i>L</i> (192, 71)  | <i>t01690</i>   | (0, 1)  | <i>L</i> (196, 75)  | <i>t01850</i>   | (1, 0)  | <i>L</i> (108, 23)  |
| <i>t01863</i>   | (0, 1)  | <i>L</i> (133, 36)  | <i>t01949</i>   | (1, 0)  | <i>L</i> (127, 29)  | <i>t02104</i>   | (0, 1)  | <i>L</i> (119, 50)  |
| <i>t02378</i>   | (0, 1)  | <i>L</i> (163, 62)  | <i>t03979</i>   | (0, 1)  | <i>L</i> (115, 34)  | <i>t04180</i>   | (0, 1)  | <i>L</i> (125, 49)  |
| <i>t04244</i>   | (1, 0)  | <i>L</i> (181, 70)  | <i>t04382</i>   | (0, 1)  | <i>L</i> (157, 46)  | <i>t04721</i>   | (1, 0)  | <i>L</i> (147, 41)  |
| <i>t05425</i>   | (0, 1)  | <i>L</i> (117, 43)  | <i>t05538</i>   | (0, 1)  | <i>L</i> (105, 41)  | <i>t05564</i>   | (0, 1)  | <i>L</i> (135, 41)  |
| <i>t05658</i>   | (1, 0)  | <i>L</i> (112, 31)  | <i>t05695</i>   | (0, 1)  | <i>L</i> (120, 49)  | <i>t06001</i>   | (1, 0)  | <i>L</i> (133, 39)  |
| <i>t08403</i>   | (0, 1)  | <i>L</i> (107, 41)  | <i>t09580</i>   | (0, 1)  | <i>L</i> (116, 45)  | <i>o9_00133</i> | (0, 1)  | <i>L</i> (132, 25)  |
| <i>o9_00168</i> | (0, 1)  | <i>L</i> (143, 25)  | <i>o9_00644</i> | (0, 1)  | <i>L</i> (72, 23)   | <i>o9_00797</i> | (-1, 1) | <i>L</i> (215, 49)  |
| <i>o9_00797</i> | (0, 1)  | <i>L</i> (214, 49)  | <i>o9_00815</i> | (-1, 1) | <i>L</i> (226, 49)  | <i>o9_00815</i> | (0, 1)  | <i>L</i> (227, 49)  |
| <i>o9_01584</i> | (0, 1)  | <i>L</i> (219, 64)  | <i>o9_01621</i> | (0, 1)  | <i>L</i> (229, 64)  | <i>o9_01680</i> | (1, 0)  | <i>L</i> (211, 64)  |
| <i>o9_01765</i> | (1, 0)  | <i>L</i> (237, 64)  | <i>o9_02255</i> | (0, 1)  | <i>L</i> (227, 84)  | <i>o9_02340</i> | (1, 0)  | <i>L</i> (237, 64)  |
| <i>o9_02350</i> | (0, 1)  | <i>L</i> (273, 100) | <i>o9_02386</i> | (1, 0)  | <i>L</i> (263, 71)  | <i>o9_02655</i> | (0, 1)  | <i>L</i> (196, 75)  |
| <i>o9_02696</i> | (0, 1)  | <i>L</i> (209, 80)  | <i>o9_02706</i> | (1, 0)  | <i>L</i> (274, 81)  | <i>o9_02735</i> | (1, 0)  | <i>L</i> (293, 81)  |
| <i>o9_02772</i> | (-1, 1) | <i>L</i> (95, 41)   | <i>o9_02786</i> | (-1, 1) | <i>L</i> (98, 37)   | <i>o9_02794</i> | (1, 1)  | <i>L</i> (110, 41)  |
| <i>o9_03108</i> | (-1, 1) | <i>L</i> (103, 46)  | <i>o9_03118</i> | (1, 0)  | <i>L</i> (292, 111) | <i>o9_03133</i> | (0, 1)  | <i>L</i> (157, 36)  |
| <i>o9_03149</i> | (1, 0)  | <i>L</i> (313, 119) | <i>o9_03162</i> | (0, 1)  | <i>L</i> (288, 119) | <i>o9_03188</i> | (0, 1)  | <i>L</i> (317, 121) |
| <i>o9_03288</i> | (1, 0)  | <i>L</i> (158, 37)  | <i>o9_03313</i> | (0, 1)  | <i>L</i> (206, 63)  | <i>o9_03412</i> | (1, 0)  | <i>L</i> (205, 61)  |
| <i>o9_03526</i> | (1, 0)  | <i>L</i> (91, 16)   | <i>o9_03802</i> | (0, 1)  | <i>L</i> (151, 45)  | <i>o9_03932</i> | (1, 0)  | <i>L</i> (135, 31)  |
| <i>o9_04313</i> | (1, 0)  | <i>L</i> (240, 71)  | <i>o9_04431</i> | (1, 0)  | <i>L</i> (267, 79)  | <i>o9_04435</i> | (1, 0)  | <i>L</i> (162, 35)  |
| <i>o9_07893</i> | (0, 1)  | <i>L</i> (199, 55)  | <i>o9_07945</i> | (0, 1)  | <i>L</i> (233, 89)  | <i>o9_08647</i> | (1, 0)  | <i>L</i> (271, 75)  |
| <i>o9_08771</i> | (1, 0)  | <i>L</i> (317, 121) | <i>o9_08828</i> | (0, 1)  | <i>L</i> (239, 70)  | <i>o9_08875</i> | (0, 1)  | <i>L</i> (268, 99)  |
| <i>o9_09213</i> | (0, 1)  | <i>L</i> (150, 59)  | <i>o9_10696</i> | (1, 0)  | <i>L</i> (101, 21)  | <i>o9_11999</i> | (1, 0)  | <i>L</i> (253, 74)  |
| <i>o9_12459</i> | (1, 0)  | <i>L</i> (148, 41)  | <i>o9_12519</i> | (0, 1)  | <i>L</i> (130, 51)  | <i>o9_12757</i> | (0, 1)  | <i>L</i> (145, 59)  |
| <i>o9_12873</i> | (0, 1)  | <i>L</i> (261, 100) | <i>o9_12971</i> | (0, 1)  | <i>L</i> (153, 55)  | <i>o9_13052</i> | (1, 0)  | <i>L</i> (172, 39)  |
| <i>o9_13125</i> | (1, 0)  | <i>L</i> (177, 49)  | <i>o9_13188</i> | (0, 1)  | <i>L</i> (171, 53)  | <i>o9_13433</i> | (0, 1)  | <i>L</i> (209, 80)  |
| <i>o9_13666</i> | (1, 0)  | <i>L</i> (191, 56)  | <i>o9_13952</i> | (0, 1)  | <i>L</i> (229, 94)  | <i>o9_14716</i> | (0, 1)  | <i>L</i> (196, 55)  |
| <i>o9_14831</i> | (-1, 1) | <i>L</i> (79, 28)   | <i>o9_18007</i> | (0, 1)  | <i>L</i> (161, 45)  | <i>o9_18209</i> | (0, 1)  | <i>L</i> (182, 53)  |
| <i>o9_21893</i> | (1, 0)  | <i>L</i> (93, 25)   | <i>o9_22129</i> | (0, 1)  | <i>L</i> (121, 35)  | <i>o9_22477</i> | (0, 1)  | <i>L</i> (97, 35)   |
| <i>o9_24534</i> | (1, 0)  | <i>L</i> (133, 30)  | <i>o9_25595</i> | (0, 1)  | <i>L</i> (139, 42)  | <i>o9_26791</i> | (0, 1)  | <i>L</i> (172, 63)  |
| <i>o9_27155</i> | (0, 1)  | <i>L</i> (161, 61)  |                 |         |                     |                 |         |                     |

TABLE 4. The integer alternating surgeries to Seifert fibered spaces with base  $S^2$  and three exceptional fibers which are not lens spaces. The column titled *filled manifold* shows the Seifert invariants in Regina's notation.

| knot   | slope   | filled manifold      | branching set | knot   | slope   | filled manifold      | branching set |
|--------|---------|----------------------|---------------|--------|---------|----------------------|---------------|
| m082   | (1, 1)  | (2, 1)(2, 1)(5, 2)   | L8a3          | m103   | (-1, 1) | (2, 1)(2, 1)(3, 8)   | L9a16         |
| m144   | (-1, 1) | (2, 1)(3, 1)(5, 2)   | K9a9          | m194   | (1, 1)  | (2, 1)(2, 1)(7, 2)   | L9a7          |
| m198   | (0, 1)  | (2, 1)(3, 1)(4, 3)   | L9a24         | m240   | (-1, 1) | (2, 1)(2, 1)(5, 4)   | L9a12         |
| m270   | (1, 1)  | (2, 1)(3, 2)(4, 3)   | L9a23         | m276   | (1, 1)  | (2, 1)(3, 2)(3, 5)   | K9a5          |
| m281   | (0, 1)  | (2, 1)(3, 2)(5, 2)   | K9a4          | s042   | (1, 1)  | (2, 1)(2, 1)(3, 11)  | L10a41        |
| s068   | (-1, 1) | (2, 1)(3, 2)(3, 8)   | K10a17        | s086   | (-1, 1) | (2, 1)(4, 1)(5, 2)   | L10a67        |
| s301   | (0, 1)  | (2, 1)(3, 1)(4, 7)   | L10a72        | s301   | (1, 1)  | (2, 1)(3, 2)(7, 2)   | K10a9         |
| s308   | (-1, 1) | (2, 1)(2, 1)(7, 9)   | L10a19        | s308   | (0, 1)  | (3, 1)(3, 2)(4, 3)   | K10a42        |
| s344   | (1, 1)  | (2, 1)(2, 1)(9, 7)   | L10a10        | s346   | (1, 1)  | (2, 1)(2, 1)(13, 5)  | L10a29        |
| s367   | (0, 1)  | (3, 1)(3, 2)(5, 2)   | K10a37        | s369   | (-1, 1) | (2, 1)(3, 2)(4, 7)   | L10a59        |
| s407   | (-1, 1) | (2, 1)(3, 2)(8, 3)   | L10a60        | s582   | (-1, 1) | (2, 1)(2, 1)(9, 4)   | L10a40        |
| s582   | (0, 1)  | (2, 1)(3, 1)(7, 3)   | K10a82        | s769   | (0, 1)  | (3, 2)(3, 2)(4, 3)   | K10a40        |
| s769   | (1, 0)  | (2, 1)(2, 1)(7, 12)  | L10a30        | v0082  | (1, 1)  | (2, 1)(3, 1)(3, 11)  | K11a58        |
| v0114  | (1, 1)  | (2, 1)(3, 2)(4, 11)  | L11a190       | v0165  | (1, 1)  | (2, 1)(5, 1)(5, 2)   | K11a62        |
| v0330  | (0, 1)  | (2, 1)(3, 1)(6, 5)   | L11a274       | v0398  | (0, 1)  | (2, 1)(3, 1)(9, 7)   | K11a118       |
| v0398  | (1, 1)  | (2, 1)(2, 1)(5, 17)  | L11a94        | v0424  | (1, 1)  | (2, 1)(4, 3)(5, 4)   | L11a186       |
| v0497  | (1, 1)  | (2, 1)(4, 3)(7, 5)   | L11a151       | v0554  | (0, 1)  | (3, 1)(3, 1)(5, 4)   | L11a383       |
| v0570  | (0, 1)  | (3, 1)(3, 1)(4, 7)   | K11a340       | v0570  | (1, 1)  | (2, 1)(4, 3)(7, 2)   | L11a154       |
| v0573  | (-1, 1) | (2, 1)(3, 1)(7, 9)   | K11a153       | v0573  | (0, 1)  | (3, 1)(4, 3)(4, 3)   | L11a296       |
| v0709  | (1, 1)  | (2, 1)(3, 1)(6, 5)   | L11a274       | v0715  | (-1, 1) | (3, 2)(3, 2)(4, 7)   | K11a107       |
| v0740  | (0, 1)  | (3, 2)(4, 1)(5, 2)   | K11a133       | v0741  | (1, 1)  | (3, 2)(3, 2)(5, 8)   | L11a268       |
| v0765  | (-1, 1) | (2, 1)(2, 1)(9, 11)  | L11a43        | v0765  | (0, 1)  | (3, 1)(3, 2)(5, 4)   | K11a201       |
| v0847  | (-1, 1) | (2, 1)(5, 2)(5, 4)   | K11a60        | v0912  | (1, 1)  | (3, 1)(3, 2)(4, 7)   | K11a139       |
| v0939  | (0, 1)  | (2, 1)(2, 1)(11, 7)  | L10a28        | v0945  | (0, 1)  | (2, 1)(3, 1)(7, 12)  | K11a94        |
| v1077  | (0, 1)  | (2, 1)(3, 2)(8, 11)  | L11a160       | v1077  | (1, 1)  | (2, 1)(3, 2)(13, 5)  | K11a35        |
| v1109  | (-1, 1) | (2, 1)(2, 1)(13, 18) | L11a113       | v1109  | (0, 1)  | (3, 2)(3, 2)(8, 3)   | K11a134       |
| v1300  | (1, 0)  | (2, 1)(4, 1)(5, 4)   | L11a200       | v1620  | (0, 1)  | (3, 1)(3, 1)(7, 3)   | K11a361       |
| v1620  | (1, 1)  | (2, 1)(2, 1)(13, 4)  | L11a75        | v1628  | (0, 1)  | (2, 1)(3, 1)(4, 11)  | L11a191       |
| v1628  | (1, 0)  | (2, 1)(5, 2)(5, 4)   | K11a60        | v1690  | (-1, 1) | (2, 1)(3, 2)(5, 8)   | K10a3         |
| v1716  | (1, 1)  | (2, 1)(2, 1)(11, 8)  | L10a25        | v1718  | (-1, 1) | (2, 1)(4, 3)(7, 3)   | L11a189       |
| v1718  | (0, 1)  | (2, 1)(5, 2)(7, 3)   | K11a63        | v1728  | (1, 1)  | (2, 1)(4, 3)(5, 3)   | L10a57        |
| v1940  | (0, 1)  | (2, 1)(4, 3)(5, 7)   | L11a155       | v1940  | (1, 0)  | (2, 1)(3, 2)(9, 7)   | K11a16        |
| v1966  | (0, 1)  | (3, 2)(4, 3)(5, 3)   | K11a87        | v1966  | (1, 0)  | (2, 1)(2, 1)(11, 19) | L11a77        |
| v2024  | (0, 1)  | (2, 1)(5, 3)(7, 3)   | K11a10        | v2024  | (1, 1)  | (2, 1)(4, 3)(5, 7)   | L11a155       |
| v2090  | (-1, 1) | (3, 2)(3, 2)(5, 7)   | K11a78        | v2090  | (0, 1)  | (2, 1)(5, 2)(8, 5)   | L11a157       |
| v2759  | (0, 1)  | (2, 1)(3, 1)(9, 4)   | K11a260       | v2759  | (1, 1)  | (2, 1)(3, 1)(10, 3)  | L11a259       |
| v3354  | (1, 1)  | (3, 2)(3, 2)(7, 3)   | K11a202       | t00110 | (1, 1)  | (2, 1)(3, 2)(4, 13)  | L12a647       |
| t00146 | (-1, 1) | (2, 1)(3, 2)(5, 14)  | K12a158       | t00324 | (-1, 1) | (2, 1)(5, 2)(6, 1)   | L12a896       |
| t00729 | (-1, 1) | (2, 1)(2, 1)(5, 22)  | L12a410       | t00729 | (0, 1)  | (2, 1)(3, 1)(11, 9)  | K12a591       |
| t00787 | (0, 1)  | (2, 1)(3, 1)(14, 11) | L12a872       | t00787 | (1, 1)  | (2, 1)(3, 2)(5, 17)  | K12a118       |
| t00873 | (1, 1)  | (2, 1)(4, 3)(9, 7)   | L12a492       | t00932 | (-1, 1) | (2, 1)(4, 3)(11, 8)  | L12a595       |
| t01033 | (0, 1)  | (3, 1)(4, 1)(4, 7)   | L12a1058      | t01033 | (1, 1)  | (2, 1)(5, 4)(7, 2)   | K12a420       |
| t01037 | (-1, 1) | (2, 1)(4, 1)(7, 9)   | L12a530       | t01037 | (0, 1)  | (3, 1)(4, 3)(5, 4)   | K12a1028      |
| t01125 | (1, 1)  | (2, 1)(2, 1)(23, 9)  | L12a339       | t01216 | (1, 1)  | (2, 1)(2, 1)(19, 15) | L12a187       |
| t01268 | (1, 1)  | (2, 1)(2, 1)(31, 12) | L12a221       | t01292 | (1, 1)  | (2, 1)(2, 1)(23, 18) | L12a327       |
| t01409 | (1, 1)  | (3, 2)(3, 2)(7, 12)  | L12a932       | t01424 | (-1, 1) | (3, 2)(3, 2)(8, 13)  | K12a281       |
| t01440 | (0, 1)  | (3, 2)(5, 1)(5, 2)   | K12a619       | t01598 | (-1, 1) | (2, 1)(3, 2)(10, 17) | L12a887       |
| t01636 | (1, 1)  | (2, 1)(3, 2)(18, 7)  | L12a888       | t01646 | (-1, 1) | (2, 1)(3, 2)(11, 19) | K12a98        |
| t01690 | (1, 1)  | (2, 1)(3, 2)(21, 8)  | K12a95        | t01757 | (-1, 1) | (2, 1)(2, 1)(9, 20)  | L12a269       |
| t01757 | (0, 1)  | (3, 1)(5, 2)(5, 4)   | K12a752       | t01834 | (-1, 1) | (2, 1)(3, 2)(9, 11)  | K12a62        |
| t01834 | (0, 1)  | (3, 1)(5, 3)(5, 4)   | L12a1323      | t01850 | (1, 1)  | (2, 1)(3, 1)(11, 9)  | K12a591       |
| t01863 | (1, 1)  | (2, 1)(3, 1)(18, 7)  | L12a889       | t01949 | (1, 1)  | (3, 1)(3, 2)(5, 9)   | L12a1292      |
| t02099 | (-1, 1) | (2, 1)(3, 1)(11, 7)  | K11a257       | t02238 | (0, 1)  | (2, 1)(3, 1)(7, 19)  | K12a238       |
| t02378 | (-1, 1) | (3, 1)(3, 2)(13, 5)  | L12a1299      | t02398 | (0, 1)  | (3, 1)(3, 2)(7, 12)  | K12a524       |
| t02404 | (0, 1)  | (2, 1)(2, 1)(19, 12) | L11a62        | t02470 | (0, 1)  | (2, 1)(3, 2)(11, 15) | K12a112       |
| t02470 | (1, 1)  | (2, 1)(3, 2)(18, 7)  | L12a888       | t02537 | (-1, 1) | (2, 1)(4, 3)(13, 5)  | L12a599       |
| t02537 | (0, 1)  | (3, 1)(3, 2)(8, 11)  | K12a445       | t02567 | (-1, 1) | (2, 1)(3, 1)(13, 18) | K12a240       |
| t02567 | (0, 1)  | (3, 2)(4, 3)(8, 3)   | L12a964       | t02639 | (0, 1)  | (3, 2)(3, 2)(13, 5)  | K12a229       |
| t02639 | (1, 1)  | (2, 1)(2, 1)(21, 29) | L12a256       | t03566 | (0, 1)  | (2, 1)(3, 1)(4, 15)  | L12a678       |
| t03566 | (1, 0)  | (2, 1)(5, 4)(7, 2)   | K12a420       | t03607 | (0, 1)  | (2, 1)(3, 1)(19, 8)  | K12a436       |
| t03607 | (1, 1)  | (2, 1)(2, 1)(25, 11) | L12a350       | t03709 | (0, 1)  | (3, 1)(3, 2)(4, 11)  | K12a376       |
| t03709 | (1, 0)  | (2, 1)(5, 4)(8, 3)   | L12a615       | t03713 | (-1, 1) | (2, 1)(3, 2)(5, 13)  | K11a11        |
| t03781 | (0, 1)  | (3, 1)(4, 1)(7, 3)   | K12a1243      | t03781 | (1, 1)  | (2, 1)(2, 1)(17, 4)  | L12a289       |
| t03864 | (1, 1)  | (3, 2)(3, 2)(5, 8)   | L11a268       | t03956 | (-1, 1) | (2, 1)(5, 3)(5, 4)   | K11a7         |
| t04003 | (-1, 1) | (2, 1)(2, 1)(11, 19) | L11a77        | t04019 | (-1, 1) | (2, 1)(3, 1)(11, 5)  | K12a843       |
| t04019 | (0, 1)  | (2, 1)(4, 1)(9, 4)   | L12a646       | t04102 | (1, 1)  | (2, 1)(3, 2)(11, 8)  | K11a31        |
| t04228 | (0, 1)  | (2, 1)(4, 3)(7, 10)  | L12a676       | t04228 | (1, 0)  | (2, 1)(3, 2)(13, 10) | K12a144       |
| t05118 | (-1, 1) | (2, 1)(5, 2)(7, 12)  | K12a175       | t05118 | (0, 1)  | (2, 1)(5, 3)(12, 5)  | L12a702       |
| t05239 | (0, 1)  | (3, 2)(4, 3)(7, 4)   | K12a368       | t05239 | (1, 0)  | (2, 1)(4, 3)(7, 12)  | L12a600       |
| t05390 | (-1, 1) | (2, 1)(4, 3)(7, 5)   | L11a151       | t05426 | (0, 1)  | (3, 2)(4, 3)(8, 5)   | L12a972       |
| t05426 | (1, 0)  | (2, 1)(5, 3)(7, 12)  | K12a21        | t05578 | (0, 1)  | (4, 3)(4, 3)(5, 3)   | L12a962       |
| t05578 | (1, 0)  | (2, 1)(3, 1)(11, 19) | K12a258       | t05663 | (0, 1)  | (3, 2)(5, 2)(5, 4)   | L12a1105      |
| t05663 | (1, 0)  | (2, 1)(3, 1)(9, 16)  | K12a329       | t05674 | (-1, 1) | (2, 1)(4, 3)(7, 9)   | L12a501       |
| t05674 | (0, 1)  | (3, 1)(5, 3)(7, 3)   | K12a749       | t06440 | (0, 1)  | (3, 2)(5, 2)(7, 3)   | K12a568       |

TABLE 5. Table 4 continued.

| knot     | slope   | filled manifold      | branching set | knot     | slope   | filled manifold      | branching set |
|----------|---------|----------------------|---------------|----------|---------|----------------------|---------------|
| t06463   | (0, 1)  | (2, 1)(5, 2)(8, 13)  | L12a516       | t06525   | (0, 1)  | (2, 1)(5, 3)(8, 5)   | L11a159       |
| t06570   | (0, 1)  | (2, 1)(5, 2)(7, 10)  | K12a194       | t06605   | (0, 1)  | (3, 2)(5, 2)(8, 5)   | K12a263       |
| t07348   | (0, 1)  | (2, 1)(3, 2)(8, 5)   | L10a61        | t08111   | (0, 1)  | (2, 1)(3, 2)(8, 3)   | L10a60        |
| t08201   | (0, 1)  | (3, 2)(3, 2)(5, 3)   | K10a38        | t08267   | (0, 1)  | (2, 1)(2, 1)(21, 13) | L11a55        |
| t09016   | (0, 1)  | (2, 1)(2, 1)(13, 21) | L11a78        | t09267   | (0, 1)  | (3, 1)(3, 2)(10, 3)  | K12a577       |
| t09313   | (0, 1)  | (2, 1)(3, 2)(16, 7)  | L12a718       | t09455   | (0, 1)  | (2, 1)(3, 1)(10, 13) | L12a926       |
| t09704   | (0, 1)  | (2, 1)(2, 1)(19, 27) | L12a292       | t09852   | (0, 1)  | (2, 1)(2, 1)(13, 5)  | L10a29        |
| t10230   | (0, 1)  | (2, 1)(2, 1)(11, 7)  | L10a28        | t10462   | (0, 1)  | (2, 1)(5, 3)(7, 5)   | K11a1         |
| t10643   | (1, 1)  | (3, 2)(3, 2)(10, 3)  | K12a648       | t10681   | (0, 1)  | (2, 1)(3, 2)(12, 17) | L12a709       |
| t10985   | (-1, 1) | (3, 2)(5, 3)(7, 3)   | L12a1286      | o9_00133 | (-1, 1) | (2, 1)(3, 2)(5, 16)  | K13a633       |
| o9_00168 | (1, 1)  | (2, 1)(3, 2)(6, 17)  | L13a2992      | o9_00644 | (-1, 1) | (2, 1)(5, 2)(7, 1)   | K13a646       |
| o9_01436 | (0, 1)  | (2, 1)(3, 1)(16, 13) | L13a4220      | o9_01436 | (1, 1)  | (2, 1)(3, 1)(5, 22)  | K13a666       |
| o9_01496 | (-1, 1) | (2, 1)(4, 3)(5, 17)  | L13a1884      | o9_01496 | (0, 1)  | (2, 1)(3, 1)(19, 15) | K13a3215      |
| o9_01680 | (1, 1)  | (2, 1)(4, 3)(13, 10) | L13a2083      | o9_01765 | (-1, 1) | (2, 1)(4, 3)(15, 11) | L13a1850      |
| o9_01953 | (0, 1)  | (3, 1)(4, 3)(5, 6)   | K13a4562      | o9_01953 | (1, 1)  | (2, 1)(6, 5)(7, 2)   | L13a2843      |
| o9_01955 | (0, 1)  | (3, 1)(4, 3)(6, 5)   | L13a4298      | o9_01955 | (1, 1)  | (2, 1)(5, 1)(7, 9)   | K13a1536      |
| o9_02255 | (1, 1)  | (2, 1)(2, 1)(41, 16) | L13a597       | o9_02340 | (-1, 1) | (2, 1)(2, 1)(33, 26) | L13a957       |
| o9_02350 | (1, 1)  | (2, 1)(2, 1)(49, 19) | L13a949       | o9_02386 | (-1, 1) | (2, 1)(2, 1)(37, 29) | L13a500       |
| o9_02706 | (-1, 1) | (3, 2)(3, 2)(10, 17) | K13a2041      | o9_02735 | (1, 1)  | (3, 2)(3, 2)(11, 18) | L13a4183      |
| o9_02772 | (0, 1)  | (3, 1)(3, 1)(7, 6)   | L13a5041      | o9_02794 | (0, 1)  | (3, 2)(5, 2)(6, 1)   | K13a2427      |
| o9_03032 | (-1, 1) | (2, 1)(2, 1)(7, 30)  | L13a1210      | o9_03032 | (0, 1)  | (3, 1)(3, 1)(11, 9)  | K13a3004      |
| o9_03108 | (0, 1)  | (3, 1)(4, 1)(6, 5)   | L13a4297      | o9_03118 | (-1, 1) | (2, 1)(3, 2)(17, 29) | K13a299       |
| o9_03149 | (1, 1)  | (2, 1)(3, 2)(18, 31) | L13a2812      | o9_03162 | (1, 1)  | (2, 1)(3, 2)(31, 12) | K13a296       |
| o9_03188 | (1, 1)  | (2, 1)(3, 2)(34, 13) | L13a2823      | o9_03288 | (1, 1)  | (2, 1)(5, 4)(9, 4)   | K13a3453      |
| o9_03412 | (1, 1)  | (2, 1)(5, 4)(12, 5)  | L13a2528      | o9_03526 | (-1, 1) | (2, 1)(4, 1)(7, 6)   | L13a2127      |
| o9_03586 | (-1, 1) | (2, 1)(3, 1)(9, 20)  | K13a1584      | o9_03586 | (0, 1)  | (3, 1)(5, 4)(7, 3)   | L13a5059      |
| o9_03622 | (-1, 1) | (2, 1)(4, 3)(9, 11)  | L13a1604      | o9_03622 | (0, 1)  | (3, 1)(5, 4)(7, 4)   | K13a4311      |
| o9_03833 | (-1, 1) | (2, 1)(2, 1)(11, 24) | L13a768       | o9_03833 | (0, 1)  | (3, 1)(5, 2)(6, 5)   | K13a2317      |
| o9_03932 | (1, 1)  | (2, 1)(6, 5)(7, 2)   | L13a2843      | o9_04106 | (0, 1)  | (3, 1)(3, 2)(13, 10) | K13a2807      |
| o9_04205 | (0, 1)  | (3, 1)(3, 2)(14, 11) | K13a2110      | o9_04245 | (0, 1)  | (2, 1)(3, 1)(15, 26) | K13a2857      |
| o9_04269 | (-1, 1) | (2, 1)(4, 1)(11, 7)  | L12a634       | o9_04313 | (1, 1)  | (3, 2)(4, 3)(7, 10)  | K13a1458      |
| o9_04431 | (1, 1)  | (3, 2)(4, 3)(8, 11)  | L13a3104      | o9_04435 | (1, 1)  | (3, 2)(4, 1)(5, 9)   | K13a1220      |
| o9_04438 | (0, 1)  | (2, 1)(3, 1)(18, 31) | L13a2960      | o9_05021 | (0, 1)  | (3, 1)(3, 1)(7, 19)  | K13a2832      |
| o9_05177 | (0, 1)  | (3, 1)(4, 3)(7, 12)  | K13a1941      | o9_05229 | (0, 1)  | (3, 1)(4, 3)(9, 7)   | K13a2122      |
| o9_05357 | (0, 1)  | (2, 1)(3, 1)(10, 27) | L13a2981      | o9_05426 | (-1, 1) | (2, 1)(5, 4)(13, 5)  | K13a817       |
| o9_05426 | (0, 1)  | (3, 2)(4, 1)(8, 11)  | L13a3443      | o9_05483 | (-1, 1) | (2, 1)(4, 1)(13, 18) | L13a2133      |
| o9_05483 | (0, 1)  | (3, 2)(5, 4)(8, 3)   | K13a1432      | o9_05562 | (0, 1)  | (3, 1)(3, 1)(11, 19) | K13a2841      |
| o9_05618 | (0, 1)  | (3, 1)(5, 3)(9, 7)   | K13a2002      | o9_05860 | (-1, 1) | (2, 1)(5, 2)(18, 7)  | L13a2837      |
| o9_05860 | (0, 1)  | (2, 1)(3, 2)(11, 26) | K13a523       | o9_05970 | (0, 1)  | (3, 1)(3, 2)(11, 19) | L13a4371      |
| o9_06060 | (0, 1)  | (2, 1)(2, 1)(19, 31) | L12a226       | o9_06128 | (-1, 1) | (2, 1)(5, 3)(18, 7)  | L13a2838      |
| o9_06128 | (0, 1)  | (3, 2)(3, 2)(11, 15) | K13a1818      | o9_06154 | (0, 1)  | (2, 1)(3, 2)(19, 12) | K12a83        |
| o9_06248 | (-1, 1) | (2, 1)(2, 1)(21, 50) | L13a1153      | o9_06248 | (0, 1)  | (3, 2)(5, 2)(13, 5)  | K13a788       |
| o9_06301 | (-1, 1) | (2, 1)(3, 2)(21, 29) | K13a332       | o9_06301 | (0, 1)  | (3, 2)(5, 3)(13, 5)  | L13a4461      |
| o9_07790 | (-1, 1) | (2, 1)(6, 5)(7, 3)   | L13a2991      | o9_07790 | (0, 1)  | (2, 1)(5, 2)(11, 5)  | K13a653       |
| o9_07943 | (0, 1)  | (3, 1)(3, 1)(4, 15)  | K13a4569      | o9_07943 | (1, 0)  | (2, 1)(5, 4)(10, 3)  | L13a2937      |
| o9_08006 | (-1, 1) | (2, 1)(7, 3)(9, 7)   | K13a1044      | o9_08006 | (0, 1)  | (2, 1)(5, 2)(16, 7)  | L13a2240      |
| o9_08042 | (0, 1)  | (3, 1)(4, 3)(4, 11)  | L13a3474      | o9_08042 | (1, 0)  | (2, 1)(5, 4)(11, 4)  | K13a3452      |
| o9_08224 | (1, 1)  | (3, 1)(3, 2)(5, 13)  | L12a1239      | o9_08302 | (1, 1)  | (3, 2)(4, 3)(5, 8)   | K12a219       |
| o9_08477 | (0, 1)  | (3, 1)(5, 1)(7, 3)   | K13a4871      | o9_08477 | (1, 1)  | (2, 1)(2, 1)(21, 4)  | L13a699       |
| o9_08765 | (-1, 1) | (2, 1)(3, 1)(11, 19) | K12a258       | o9_08776 | (0, 1)  | (3, 2)(4, 3)(11, 7)  | K13a1209      |
| o9_08776 | (1, 0)  | (2, 1)(2, 1)(25, 43) | L13a1062      | o9_08831 | (-1, 1) | (2, 1)(4, 3)(11, 8)  | L12a595       |
| o9_08852 | (0, 1)  | (3, 2)(4, 3)(13, 8)  | K13a1205      | o9_08852 | (1, 0)  | (2, 1)(2, 1)(29, 50) | L13a996       |
| o9_09465 | (-1, 1) | (3, 2)(5, 2)(5, 9)   | K13a1850      | o9_09465 | (0, 1)  | (2, 1)(5, 2)(14, 9)  | L13a2859      |
| o9_09808 | (-1, 1) | (3, 2)(5, 2)(7, 12)  | L13a3286      | o9_09808 | (0, 1)  | (2, 1)(5, 2)(19, 12) | K13a565       |
| o9_10696 | (0, 1)  | (3, 1)(4, 1)(6, 5)   | L13a4297      | o9_11248 | (1, 0)  | (2, 1)(7, 3)(10, 3)  | L13a2940      |
| o9_11248 | (1, 1)  | (2, 1)(7, 3)(9, 4)   | K13a3593      | o9_11467 | (0, 1)  | (3, 2)(4, 3)(12, 7)  | L13a3188      |
| o9_11467 | (1, 0)  | (2, 1)(7, 5)(7, 12)  | K13a809       | o9_11560 | (0, 1)  | (3, 2)(4, 3)(13, 8)  | K13a1205      |
| o9_11560 | (1, 0)  | (2, 1)(7, 5)(8, 13)  | L13a1896      | o9_11570 | (0, 1)  | (3, 1)(5, 2)(9, 4)   | K13a2804      |
| o9_11570 | (1, 1)  | (2, 1)(5, 4)(10, 3)  | L13a2937      | o9_11685 | (1, 1)  | (2, 1)(3, 1)(14, 11) | L12a872       |
| o9_11795 | (-1, 1) | (2, 1)(2, 1)(17, 14) | L12a326       | o9_11845 | (-1, 1) | (3, 1)(5, 3)(5, 4)   | L12a1323      |
| o9_12144 | (0, 1)  | (3, 1)(4, 3)(7, 10)  | K13a4563      | o9_12144 | (1, 0)  | (2, 1)(4, 3)(13, 10) | L13a2083      |
| o9_12230 | (0, 1)  | (4, 3)(4, 3)(7, 4)   | L13a3468      | o9_12230 | (1, 0)  | (2, 1)(3, 1)(15, 26) | K13a2857      |
| o9_12412 | (1, 1)  | (2, 1)(3, 2)(14, 11) | L12a870       | o9_12693 | (-1, 1) | (2, 1)(3, 1)(16, 5)  | L13a4353      |
| o9_12693 | (0, 1)  | (3, 1)(4, 1)(9, 4)   | K13a4273      | o9_12736 | (0, 1)  | (3, 1)(3, 2)(11, 9)  | L13a3633      |
| o9_12736 | (1, 0)  | (2, 1)(5, 4)(7, 9)   | K13a1390      | o9_12892 | (-1, 1) | (3, 1)(3, 2)(7, 12)  | K12a524       |
| o9_12919 | (-1, 1) | (4, 3)(4, 3)(5, 3)   | L12a962       | o9_13056 | (0, 1)  | (3, 2)(5, 4)(8, 3)   | K13a1432      |
| o9_13056 | (1, 0)  | (2, 1)(3, 1)(14, 25) | L13a2954      | o9_13182 | (-1, 1) | (2, 1)(4, 3)(9, 7)   | L12a492       |
| o9_13400 | (-1, 1) | (3, 1)(5, 2)(5, 9)   | L13a4477      | o9_13400 | (0, 1)  | (2, 1)(7, 4)(9, 4)   | K13a3456      |
| o9_13403 | (-1, 1) | (3, 2)(3, 2)(7, 12)  | L12a932       | o9_13508 | (0, 1)  | (4, 3)(4, 3)(5, 7)   | L13a3090      |
| o9_13508 | (1, 0)  | (2, 1)(7, 4)(9, 7)   | K13a1042      | o9_13537 | (-1, 1) | (4, 3)(5, 3)(5, 3)   | K12a215       |
| o9_13604 | (-1, 1) | (2, 1)(4, 3)(9, 11)  | L13a1604      | o9_13604 | (0, 1)  | (4, 1)(5, 3)(7, 3)   | K13a878       |
| o9_13639 | (0, 1)  | (2, 1)(3, 2)(17, 10) | K12a145       | o9_13649 | (1, 1)  | (2, 1)(3, 2)(9, 16)  | K12a81        |
| o9_13720 | (0, 1)  | (3, 1)(3, 2)(19, 8)  | K13a2004      | o9_14018 | (0, 1)  | (4, 3)(5, 2)(5, 8)   | K13a759       |
| o9_14018 | (1, 0)  | (2, 1)(8, 5)(9, 7)   | L13a1624      | o9_14079 | (-1, 1) | (3, 2)(4, 3)(7, 9)   | K13a937       |
| o9_14079 | (0, 1)  | (3, 1)(5, 2)(11, 7)  | L13a4350      | o9_14136 | (0, 1)  | (3, 1)(5, 2)(6, 5)   | K13a2317      |
| o9_14136 | (1, 0)  | (2, 1)(4, 1)(5, 14)  | L13a2143      | o9_14376 | (0, 1)  | (2, 1)(3, 1)(19, 27) | K13a1572      |
| o9_14599 | (-1, 1) | (4, 3)(5, 2)(5, 7)   | K13a1248      | o9_14599 | (0, 1)  | (2, 1)(7, 3)(12, 7)  | L13a2383      |
| o9_14974 | (0, 1)  | (3, 2)(5, 2)(9, 4)   | L13a3322      | o9_15633 | (0, 1)  | (2, 1)(5, 3)(13, 8)  | K12a17        |

TABLE 6. Table 5 continued.

| knot     | slope   | filled manifold      | branching set | knot     | slope   | filled manifold      | branching set |
|----------|---------|----------------------|---------------|----------|---------|----------------------|---------------|
| o9_15997 | (0, 1)  | (3, 2)(5, 2)(11, 7)  | K13a2033      | o9_16065 | (0, 1)  | (2, 1)(5, 2)(13, 21) | K13a581       |
| o9_16141 | (0, 1)  | (2, 1)(5, 3)(12, 17) | L13a2527      | o9_16157 | (0, 1)  | (3, 1)(5, 2)(8, 13)  | K13a1470      |
| o9_16181 | (0, 1)  | (2, 1)(5, 2)(12, 17) | L13a2226      | o9_16319 | (0, 1)  | (4, 3)(5, 2)(8, 5)   | L13a3098      |
| o9_16356 | (0, 1)  | (4, 3)(5, 2)(7, 3)   | K13a1469      | o9_16527 | (0, 1)  | (3, 1)(5, 2)(7, 10)  | K13a3098      |
| o9_16642 | (0, 1)  | (3, 2)(5, 3)(12, 5)  | K13a769       | o9_16748 | (0, 1)  | (3, 1)(5, 3)(8, 5)   | K12a220       |
| o9_16920 | (-1, 1) | (2, 1)(3, 2)(5, 13)  | K11a11        | o9_17450 | (-1, 1) | (3, 2)(4, 3)(7, 5)   | K12a275       |
| o9_18813 | (0, 1)  | (2, 1)(3, 2)(13, 8)  | K11a32        | o9_19130 | (0, 1)  | (2, 1)(3, 2)(11, 7)  | K11a34        |
| o9_20219 | (0, 1)  | (2, 1)(2, 1)(29, 18) | L12a331       | o9_21918 | (0, 1)  | (3, 1)(3, 2)(8, 3)   | K11a108       |
| o9_22607 | (0, 1)  | (2, 1)(4, 1)(13, 4)  | L13a1949      | o9_22607 | (1, 1)  | (3, 1)(3, 1)(11, 5)  | K13a4839      |
| o9_22663 | (-1, 1) | (3, 2)(3, 2)(8, 5)   | K11a100       | o9_22698 | (0, 1)  | (2, 1)(2, 1)(13, 34) | L12a367       |
| o9_22925 | (0, 1)  | (2, 1)(5, 2)(8, 5)   | L11a157       | o9_23023 | (0, 1)  | (2, 1)(3, 2)(13, 21) | K12a99        |
| o9_23263 | (0, 1)  | (2, 1)(7, 3)(9, 4)   | K13a3593      | o9_23660 | (0, 1)  | (2, 1)(8, 3)(9, 4)   | L13a1894      |
| o9_23955 | (0, 1)  | (3, 1)(4, 3)(10, 3)  | L13a4275      | o9_23961 | (1, 1)  | (2, 1)(3, 1)(7, 24)  | K13a3136      |
| o9_23977 | (0, 1)  | (2, 1)(7, 3)(8, 5)   | L12a626       | o9_24149 | (0, 1)  | (3, 1)(3, 1)(10, 13) | K13a4830      |
| o9_24183 | (1, 0)  | (2, 1)(2, 1)(31, 44) | L13a1362      | o9_24592 | (0, 1)  | (2, 1)(3, 2)(11, 3)  | K11a33        |
| o9_24886 | (-1, 1) | (3, 2)(7, 3)(8, 5)   | K13a1227      | o9_24889 | (0, 1)  | (2, 1)(7, 3)(7, 10)  | K13a3134      |
| o9_27261 | (0, 1)  | (2, 1)(2, 1)(29, 21) | L12a188       | o9_27392 | (0, 1)  | (2, 1)(3, 2)(23, 7)  | K13a238       |
| o9_27480 | (0, 1)  | (2, 1)(5, 2)(13, 4)  | K13a578       | o9_27737 | (1, 1)  | (2, 1)(3, 1)(13, 16) | K13a3111      |
| o9_28113 | (1, 1)  | (3, 2)(3, 2)(13, 3)  | K13a2882      | o9_28153 | (0, 1)  | (2, 1)(5, 3)(7, 12)  | K12a21        |
| o9_28529 | (1, 0)  | (2, 1)(5, 3)(16, 7)  | L13a2219      | o9_28592 | (-1, 1) | (3, 2)(5, 2)(9, 4)   | L13a3322      |
| o9_28746 | (0, 1)  | (2, 1)(3, 2)(17, 12) | K12a82        | o9_28810 | (0, 1)  | (3, 2)(5, 3)(7, 5)   | L12a1072      |
| o9_29246 | (0, 1)  | (2, 1)(2, 1)(27, 35) | L13a710       | o9_29436 | (1, 1)  | (4, 3)(5, 3)(7, 3)   | K13a842       |
| o9_30375 | (0, 1)  | (2, 1)(5, 2)(8, 13)  | L12a516       | o9_30790 | (1, 1)  | (3, 2)(5, 2)(7, 10)  | L13a4191      |
| o9_32257 | (0, 1)  | (2, 1)(3, 1)(11, 7)  | K11a257       | o9_35682 | (0, 1)  | (2, 1)(2, 1)(19, 8)  | L11a89        |
| o9_35772 | (0, 1)  | (2, 1)(2, 1)(17, 10) | L11a109       |          |         |                      |               |

TABLE 7. The integer alternating surgeries to Seifert fibered spaces with base  $\mathbb{R}P^2$  and two exceptional fibers which are not lens spaces. The row with the title filled manifold shows the Seifert invariants in Regina's notation.

| knot     | slope   | filled manifold | branching set | knot     | slope   | filled manifold | branching set |
|----------|---------|-----------------|---------------|----------|---------|-----------------|---------------|
| s684     | (1, 1)  | (2, 1)(7, -5)   | L9a3          | v1709    | (-1, 1) | (2, 1)(11, -8)  | L10a4         |
| v1980    | (-1, 1) | (3, 1)(4, -1)   | L9a9          | t11852   | (0, 1)  | (3, 1)(7, -4)   | L10a49        |
| o9_07893 | (-1, 1) | (2, 1)(25, -18) | L12a29        | o9_07945 | (-1, 1) | (2, 1)(29, -21) | L12a26        |
| o9_14831 | (0, 1)  | (4, 1)(5, -1)   | L11a51        | o9_16920 | (0, 1)  | (4, 1)(7, -2)   | L11a54        |
| o9_19130 | (1, 1)  | (3, 1)(10, -7)  | L11a102       | o9_22663 | (0, 1)  | (5, 2)(7, -5)   | L11a104       |
| o9_29529 | (0, 1)  | (2, 1)(19, -11) | L11a3         | o9_34403 | (0, 1)  | (4, 1)(7, -4)   | L11a50        |
| o9_37941 | (0, 1)  | (3, 1)(10, -7)  | L11a102       |          |         |                 |               |

TABLE 8. Integer alternating surgeries to graph manifolds. All are obtained by gluing together two Seifert fibered spaces with base  $D^2$  and with 2 exceptional fibers. The columns titled *filled manifold* gives Regina's notation for the graph manifold.

| knot  | slope   | filled manifold | branching set                     |
|-------|---------|-----------------|-----------------------------------|
| m239  | (-1, 1) | (2, 1)(3, 1)    | (2, 1)(3, 1) [-1, 1 0, 1] K8a15   |
| s294  | (-1, 1) | (2, 1)(3, 1)    | (2, 1)(4, 1) [-1, 1 0, 1] L9a22   |
| s336  | (-2, 1) | (2, 1)(3, 1)    | (3, 1)(3, 1) [-1, 1 0, 1] K9a31   |
| s665  | (1, 1)  | (2, 1)(2, 1)    | (2, 1)(3, 2) [0, -1 1, 1] L10a13  |
| s800  | (-1, 1) | (2, 1)(3, 1)    | (2, 1)(3, 2) [0, -1 1, 0] K10a8   |
| v0407 | (1, 1)  | (2, 1)(2, 1)    | (2, 1)(3, 1) [0, -1 1, 2] L11a36  |
| v0434 | (-1, 1) | (2, 1)(2, 1)    | (2, 1)(3, 2) [0, -1 1, 2] L11a35  |
| v0707 | (-2, 1) | (2, 1)(3, 1)    | (3, 1)(4, 1) [-1, 1 0, 1] K10a101 |
| v0759 | (-1, 1) | (2, 1)(2, 1)    | (2, 1)(3, 1) [2, 1  -1, 0] L11a85 |
| v0939 | (-1, 1) | (2, 1)(3, 1)    | (3, 2)(4, 1) [-1, 1 0, 1] K10a91  |
| v0945 | (1, 1)  | (2, 1)(2, 1)    | (2, 1)(3, 2) [2, 1  -1, 0] L11a84 |
| v1810 | (-1, 1) | (2, 1)(3, 1)    | (2, 1)(3, 2) [0, -1 1, 1] K11a22  |
| v1832 | (1, 1)  | (2, 1)(4, 1)    | (2, 1)(5, 3) [-1, 1 0, 1] L10a55  |
| v1839 | (-1, 1) | (2, 1)(2, 1)    | (3, 2)(3, 2) [0, -1 1, 1] L11a57  |
| v1921 | (-1, 1) | (2, 1)(3, 1)    | (2, 1)(4, 3) [0, -1 1, 0] L11a153 |
| v1986 | (-1, 1) | (2, 1)(2, 1)    | (2, 1)(7, 2) [0, -1 1, 0] L11a26  |
| v2215 | (1, 1)  | (2, 1)(3, 1)    | (2, 1)(7, 2) [-1, 1 0, 1] K10a39  |
| v2325 | (-1, 1) | (2, 1)(3, 2)    | (3, 1)(3, 1) [0, -1 1, 0] L11a315 |
| v2930 | (-1, 1) | (2, 1)(3, 1)    | (2, 1)(4, 1) [0, -1 1, 0] L11a164 |

TABLE 9. Table 8 continued.

| knot              | slope   | filled manifold |               |                  | branching set |
|-------------------|---------|-----------------|---------------|------------------|---------------|
| $v3354$           | (0, 1)  | (2, 1)(2, 1)    | (2, 1)(5, 2)  | $[1, 1] - 1, 0]$ | $L11a39$      |
| $t00826$          | (1, 1)  | (2, 1)(2, 1)    | (2, 1)(5, 2)  | $[0, -1]1, 2]$   | $L12a100$     |
| $t00855$          | (-1, 1) | (2, 1)(2, 1)    | (2, 1)(5, 3)  | $[0, -1]1, 2]$   | $L12a97$      |
| $t01318$          | (1, 1)  | (2, 1)(3, 1)    | (2, 1)(10, 3) | $[-1, 1]0, 1]$   | $L11a257$     |
| $t01368$          | (1, 1)  | (2, 1)(3, 1)    | (2, 1)(11, 3) | $[-1, 1]0, 1]$   | $K11a81$      |
| $t01422$          | (-2, 1) | (2, 1)(3, 1)    | (3, 1)(5, 1)  | $[-1, 1]0, 1]$   | $K11a323$     |
| $t02099$          | (-2, 1) | (2, 1)(3, 1)    | (4, 1)(4, 3)  | $[-1, 1]0, 1]$   | $L11a255$     |
| $t02104$          | (-1, 1) | (2, 1)(3, 1)    | (3, 1)(7, 2)  | $[-1, 1]0, 1]$   | $L11a234$     |
| $t02238$          | (-1, 1) | (2, 1)(2, 1)    | (2, 1)(5, 2)  | $[2, 1] - 1, 0]$ | $L12a240$     |
| $t02398$          | (-1, 1) | (2, 1)(2, 1)    | (2, 1)(5, 3)  | $[2, 1] - 1, 0]$ | $L12a239$     |
| $t02404$          | (-1, 1) | (2, 1)(3, 1)    | (3, 2)(7, 2)  | $[-1, 1]0, 1]$   | $K11a150$     |
| $t03979$          | (-1, 1) | (2, 1)(4, 1)    | (2, 1)(7, 4)  | $[-1, 1]0, 1]$   | $L11a144$     |
| $t04180$          | (-1, 1) | (2, 1)(3, 2)    | (2, 1)(4, 1)  | $[1, 1] - 1, 0]$ | $L12a524$     |
| $t04244$          | (1, 1)  | (2, 1)(2, 1)    | (2, 1)(7, 5)  | $[0, -1]1, 1]$   | $L12a93$      |
| $t04382$          | (1, 1)  | (2, 1)(2, 1)    | (2, 1)(11, 3) | $[0, -1]1, 0]$   | $L12a90$      |
| $t04721$          | (1, 1)  | (2, 1)(2, 1)    | (3, 1)(4, 3)  | $[0, -1]1, 1]$   | $L12a250$     |
| $t05425$          | (1, 1)  | (2, 1)(4, 1)    | (3, 1)(5, 3)  | $[-1, 1]0, 1]$   | $L11a212$     |
| $t05538$          | (-1, 1) | (2, 1)(4, 1)    | (2, 1)(7, 2)  | $[-1, 1]0, 1]$   | $L11a148$     |
| $t05564$          | (-1, 1) | (2, 1)(2, 1)    | (3, 1)(7, 2)  | $[0, -1]1, 0]$   | $L12a202$     |
| $t05658$          | (1, 1)  | (2, 1)(3, 1)    | (2, 1)(9, 7)  | $[-1, 1]0, 1]$   | $K11a167$     |
| $t05695$          | (-1, 1) | (2, 1)(3, 2)    | (3, 1)(4, 1)  | $[0, -1]1, 0]$   | $K12a93$      |
| $t06001$          | (-1, 1) | (2, 1)(4, 1)    | (2, 1)(5, 2)  | $[0, -1]1, 0]$   | $L12a523$     |
| $t06440$          | (-1, 1) | (2, 1)(3, 1)    | (2, 1)(4, 3)  | $[1, 1] - 1, 0]$ | $L12a497$     |
| $t06463$          | (1, 1)  | (2, 1)(3, 2)    | (3, 2)(3, 2)  | $[0, -1]1, 1]$   | $K12a79$      |
| $t06525$          | (1, 1)  | (2, 1)(3, 1)    | (2, 1)(11, 8) | $[-1, 1]0, 1]$   | $K11a80$      |
| $t06570$          | (-1, 1) | (2, 1)(4, 3)    | (3, 1)(3, 2)  | $[0, -1]1, 0]$   | $L12a602$     |
| $t06605$          | (1, 1)  | (2, 1)(2, 1)    | (3, 2)(3, 2)  | $[-1, -1]2, 1]$  | $L12a342$     |
| $t07348$          | (-1, 1) | (2, 1)(5, 2)    | (3, 1)(3, 1)  | $[-1, 1]0, 1]$   | $K10a12$      |
| $t08111$          | (-1, 1) | (2, 1)(3, 1)    | (3, 1)(4, 3)  | $[-1, 1]0, 1]$   | $K10a106$     |
| $t08201$          | (1, 1)  | (2, 1)(3, 1)    | (3, 1)(5, 2)  | $[-1, 1]0, 1]$   | $L10a84$      |
| $t08267$          | (1, 1)  | (2, 1)(3, 1)    | (2, 1)(11, 8) | $[-1, 1]0, 1]$   | $K11a80$      |
| $t08403$          | (-1, 1) | (2, 1)(4, 1)    | (2, 1)(7, 2)  | $[-1, 1]0, 1]$   | $L11a148$     |
| $t09016$          | (-1, 1) | (2, 1)(5, 2)    | (2, 1)(7, 2)  | $[-1, 1]0, 1]$   | $K11a52$      |
| $t09267$          | (1, 1)  | (2, 1)(3, 1)    | (2, 1)(4, 1)  | $[0, -1]1, 1]$   | $L12a529$     |
| $t09313$          | (1, 1)  | (2, 1)(3, 1)    | (2, 1)(5, 2)  | $[0, -1]1, 1]$   | $K12a129$     |
| $t09455$          | (-1, 1) | (2, 1)(3, 1)    | (3, 2)(4, 1)  | $[0, -1]1, 0]$   | $K12a355$     |
| $t09704$          | (-1, 1) | (2, 1)(3, 1)    | (3, 2)(5, 3)  | $[0, -1]1, 0]$   | $K12a271$     |
| $t09852$          | (1, 1)  | (2, 1)(3, 1)    | (3, 1)(4, 3)  | $[-1, 1]0, 1]$   | $K10a106$     |
| $t09954$          | (-1, 1) | (2, 1)(4, 1)    | (2, 1)(5, 3)  | $[-1, 1]0, 1]$   | $L10a55$      |
| $t09954$          | (0, 1)  | (2, 1)(3, 1)    | (2, 1)(7, 3)  | $[-1, 1]0, 1]$   | $K10a87$      |
| $t10188$          | (0, 1)  | (2, 1)(3, 1)    | (2, 1)(5, 2)  | $[-1, 1]0, 1]$   | $K9a6$        |
| $t10643$          | (0, 1)  | (2, 1)(2, 1)    | (3, 1)(5, 2)  | $[1, 1] - 1, 0]$ | $L12a363$     |
| $t10681$          | (-1, 1) | (2, 1)(3, 1)    | (3, 2)(5, 3)  | $[0, -1]1, 0]$   | $K12a271$     |
| $t10985$          | (0, 1)  | (2, 1)(3, 2)    | (2, 1)(5, 2)  | $[1, 1] - 1, 0]$ | $K12a57$      |
| $t12753$          | (0, 1)  | (2, 1)(3, 1)    | (3, 2)(5, 3)  | $[-1, 1]0, 1]$   | $L10a85$      |
| $\text{o9.01584}$ | (-1, 1) | (2, 1)(2, 1)    | (2, 1)(7, 3)  | $[0, -1]1, 2]$   | $L13a339$     |
| $\text{o9.01621}$ | (1, 1)  | (2, 1)(2, 1)    | (2, 1)(7, 4)  | $[0, -1]1, 2]$   | $L13a337$     |
| $\text{o9.02655}$ | (-1, 1) | (2, 1)(3, 1)    | (2, 1)(17, 5) | $[-1, 1]0, 1]$   | $K12a527$     |
| $\text{o9.02696}$ | (-1, 1) | (2, 1)(3, 1)    | (2, 1)(18, 5) | $[-1, 1]0, 1]$   | $L12a920$     |
| $\text{o9.02786}$ | (-2, 1) | (2, 1)(3, 1)    | (3, 1)(6, 1)  | $[-1, 1]0, 1]$   | $K12a1095$    |
| $\text{o9.03133}$ | (1, 1)  | (2, 1)(3, 1)    | (2, 1)(4, 1)  | $[0, -1]1, 2]$   | $L13a1959$    |
| $\text{o9.03313}$ | (1, 1)  | (2, 1)(3, 1)    | (2, 1)(5, 2)  | $[0, -1]1, 2]$   | $K13a587$     |
| $\text{o9.03802}$ | (-1, 1) | (2, 1)(3, 1)    | (2, 1)(4, 1)  | $[2, 1] - 1, 0]$ | $L13a1665$    |
| $\text{o9.04106}$ | (1, 1)  | (2, 1)(2, 1)    | (2, 1)(3, 1)  | $[-1, -1]4, 3]$  | $L13a380$     |
| $\text{o9.04205}$ | (1, 1)  | (2, 1)(2, 1)    | (2, 1)(3, 2)  | $[-1, -1]4, 3]$  | $L13a365$     |
| $\text{o9.04245}$ | (-1, 1) | (2, 1)(3, 2)    | (2, 1)(4, 3)  | $[0, -1]1, 2]$   | $L13a1869$    |
| $\text{o9.04269}$ | (-2, 1) | (2, 1)(3, 1)    | (4, 1)(5, 4)  | $[-1, 1]0, 1]$   | $K12a1011$    |
| $\text{o9.04438}$ | (-1, 1) | (2, 1)(3, 2)    | (2, 1)(5, 3)  | $[0, -1]1, 2]$   | $K13a60$      |
| $\text{o9.05021}$ | (-1, 1) | (2, 1)(2, 1)    | (2, 1)(7, 3)  | $[2, 1] - 1, 0]$ | $L13a765$     |
| $\text{o9.05177}$ | (-1, 1) | (2, 1)(2, 1)    | (2, 1)(7, 4)  | $[2, 1] - 1, 0]$ | $L13a763$     |
| $\text{o9.05229}$ | (-1, 1) | (2, 1)(2, 1)    | (2, 1)(3, 1)  | $[-3, -1]4, 1]$  | $L13a841$     |
| $\text{o9.05357}$ | (-1, 1) | (2, 1)(3, 1)    | (2, 1)(5, 2)  | $[2, 1] - 1, 0]$ | $K13a427$     |
| $\text{o9.05562}$ | (-1, 1) | (2, 1)(3, 2)    | (2, 1)(4, 3)  | $[2, 1] - 1, 0]$ | $L13a1595$    |
| $\text{o9.05618}$ | (-1, 1) | (2, 1)(2, 1)    | (2, 1)(3, 2)  | $[-3, -1]4, 1]$  | $L13a790$     |
| $\text{o9.05970}$ | (-1, 1) | (2, 1)(3, 2)    | (2, 1)(5, 3)  | $[2, 1] - 1, 0]$ | $K13a18$      |
| $\text{o9.06060}$ | (1, 1)  | (2, 1)(3, 1)    | (5, 2)(7, 2)  | $[-1, 1]0, 1]$   | $K12a318$     |
| $\text{o9.06154}$ | (1, 1)  | (2, 1)(3, 1)    | (5, 3)(7, 2)  | $[-1, 1]0, 1]$   | $L12a835$     |
| $\text{o9.08647}$ | (1, 1)  | (2, 1)(2, 1)    | (3, 2)(7, 4)  | $[0, -1]1, 1]$   | $L13a947$     |
| $\text{o9.08771}$ | (1, 1)  | (2, 1)(2, 1)    | (3, 2)(8, 5)  | $[0, -1]1, 1]$   | $L13a574$     |
| $\text{o9.08828}$ | (-1, 1) | (2, 1)(3, 1)    | (2, 1)(10, 7) | $[0, -1]1, 0]$   | $L13a2834$    |
| $\text{o9.08875}$ | (-1, 1) | (2, 1)(3, 1)    | (2, 1)(11, 8) | $[0, -1]1, 0]$   | $K13a803$     |
| $\text{o9.09213}$ | (1, 1)  | (2, 1)(3, 2)    | (2, 1)(5, 1)  | $[1, 1] - 1, 0]$ | $K13a176$     |
| $\text{o9.11999}$ | (1, 1)  | (2, 1)(2, 1)    | (4, 3)(5, 2)  | $[0, -1]1, 1]$   | $L13a572$     |
| $\text{o9.12459}$ | (-1, 1) | (2, 1)(5, 1)    | (2, 1)(7, 5)  | $[-1, 1]0, 1]$   | $K12a440$     |
| $\text{o9.12519}$ | (-1, 1) | (2, 1)(5, 1)    | (2, 1)(7, 2)  | $[-1, 1]0, 1]$   | $K12a365$     |
| $\text{o9.12757}$ | (-1, 1) | (2, 1)(3, 2)    | (3, 1)(5, 1)  | $[0, -1]1, 0]$   | $L13a4367$    |
| $\text{o9.12873}$ | (-1, 1) | (2, 1)(3, 1)    | (3, 2)(5, 3)  | $[0, -1]1, 1]$   | $L13a3024$    |
| $\text{o9.12971}$ | (-1, 1) | (2, 1)(4, 1)    | (4, 1)(5, 3)  | $[-1, 1]0, 1]$   | $L12a558$     |
| $\text{o9.13052}$ | (-1, 1) | (2, 1)(3, 1)    | (2, 1)(9, 2)  | $[0, -1]1, 0]$   | $K13a1413$    |

TABLE 10. Table 9 continued.

| knot     | slope   | filled manifold |                | branching set   |          |
|----------|---------|-----------------|----------------|-----------------|----------|
| 09_13125 | (1, 1)  | (2, 1)(3, 1)    | (2, 1)(14, 11) | $[-1, 1 0, 1]$  | L12a841  |
| 09_13188 | (-1, 1) | (2, 1)(2, 1)    | (4, 1)(7, 2)   | $[0, -1 1, 0]$  | L13a674  |
| 09_13433 | (1, 1)  | (2, 1)(3, 1)    | (2, 1)(18, 5)  | $[-1, 1 0, 1]$  | L12a920  |
| 09_13639 | (1, 1)  | (2, 1)(4, 1)    | (3, 2)(7, 4)   | $[-1, 1 0, 1]$  | L12a689  |
| 09_13666 | (1, 1)  | (2, 1)(4, 1)    | (2, 1)(7, 3)   | $[0, -1 1, 0]$  | L13a1663 |
| 09_13720 | (1, 1)  | (2, 1)(2, 1)    | (2, 1)(11, 3)  | $[0, -1 1, 1]$  | L13a318  |
| 09_13952 | (1, 1)  | (2, 1)(7, 5)    | (3, 1)(3, 1)   | $[0, -1 1, 0]$  | L13a3554 |
| 09_14364 | (-1, 1) | (2, 1)(2, 1)    | (2, 1)(5, 4)   | $[1, 1 0, -1]$  | L12a62   |
| 09_14376 | (1, 1)  | (2, 1)(2, 1)    | (3, 2)(11, 3)  | $[0, -1 1, 0]$  | L13a1116 |
| 09_14495 | (-1, 1) | (2, 1)(2, 1)    | (2, 1)(3, 2)   | $[-1, -1 2, 3]$ | L12a66   |
| 09_14716 | (-1, 1) | (2, 1)(3, 1)    | (3, 1)(4, 3)   | $[0, -1 1, 1]$  | K13a3243 |
| 09_14974 | (1, 1)  | (2, 1)(3, 1)    | (2, 1)(5, 4)   | $[1, 1  -1, 0]$ | K13a1545 |
| 09_15506 | (1, 1)  | (2, 1)(2, 1)    | (2, 1)(3, 2)   | $[-2, -1 3, 2]$ | L12a176  |
| 09_15633 | (1, 1)  | (2, 1)(3, 1)    | (2, 1)(18, 13) | $[-1, 1 0, 1]$  | L12a921  |
| 09_15997 | (-1, 1) | (2, 1)(2, 1)    | (3, 2)(4, 3)   | $[-1, -1 2, 1]$ | L13a707  |
| 09_16065 | (-1, 1) | (2, 1)(3, 2)    | (3, 2)(5, 3)   | $[0, -1 1, 1]$  | L13a2968 |
| 09_16141 | (-1, 1) | (2, 1)(3, 2)    | (2, 1)(7, 5)   | $[0, -1 1, 1]$  | K13a148  |
| 09_16157 | (-1, 1) | (2, 1)(4, 3)    | (3, 2)(3, 2)   | $[0, -1 1, 1]$  | L13a1842 |
| 09_16181 | (1, 1)  | (2, 1)(7, 5)    | (3, 1)(3, 2)   | $[0, -1 1, 0]$  | K13a811  |
| 09_16319 | (-1, 1) | (2, 1)(3, 1)    | (3, 2)(3, 2)   | $[-1, -1 2, 1]$ | K13a719  |
| 09_16356 | (1, 1)  | (2, 1)(4, 3)    | (3, 1)(3, 1)   | $[0, -1 1, 1]$  | L13a2089 |
| 09_16527 | (1, 1)  | (2, 1)(4, 3)    | (3, 1)(4, 3)   | $[0, -1 1, 0]$  | L13a1858 |
| 09_16642 | (-1, 1) | (2, 1)(2, 1)    | (2, 1)(7, 5)   | $[-1, -1 2, 1]$ | L13a354  |
| 09_16748 | (-1, 1) | (2, 1)(4, 1)    | (2, 1)(11, 8)  | $[-1, 1 0, 1]$  | L12a473  |
| 09_18007 | (-1, 1) | (2, 1)(9, 2)    | (3, 1)(3, 2)   | $[-1, 1 0, 1]$  | L12a536  |
| 09_18209 | (1, 1)  | (2, 1)(5, 2)    | (3, 1)(4, 1)   | $[0, -1 1, 0]$  | K13a575  |
| 09_18633 | (-1, 1) | (2, 1)(2, 1)    | (3, 2)(4, 3)   | $[1, 1 0, -1]$  | L12a184  |
| 09_18813 | (1, 1)  | (2, 1)(8, 3)    | (3, 1)(3, 1)   | $[-1, 1 0, 1]$  | L11a198  |
| 09_20219 | (-1, 1) | (2, 1)(3, 1)    | (2, 1)(15, 11) | $[-1, 1 0, 1]$  | K12a849  |
| 09_21893 | (-1, 1) | (2, 1)(3, 1)    | (3, 1)(5, 4)   | $[-1, 1 0, 1]$  | L11a282  |
| 09_21918 | (-1, 1) | (2, 1)(4, 1)    | (3, 1)(4, 3)   | $[-1, 1 0, 1]$  | L11a173  |
| 09_22129 | (-1, 1) | (2, 1)(4, 1)    | (2, 1)(5, 1)   | $[0, -1 1, 0]$  | L13a1662 |
| 09_22477 | (-1, 1) | (2, 1)(3, 1)    | (4, 1)(4, 3)   | $[-1, 1 0, 1]$  | L11a255  |
| 09_22698 | (1, 1)  | (2, 1)(7, 2)    | (2, 1)(7, 2)   | $[-1, 1 0, 1]$  | K12a353  |
| 09_22925 | (-1, 1) | (3, 1)(3, 1)    | (3, 1)(5, 2)   | $[-1, 1 0, 1]$  | K11a232  |
| 09_23023 | (1, 1)  | (2, 1)(7, 2)    | (2, 1)(8, 3)   | $[-1, 1 0, 1]$  | L12a456  |
| 09_23263 | (1, 1)  | (2, 1)(3, 1)    | (3, 1)(3, 1)   | $[0, -1 1, 2]$  | L13a4177 |
| 09_23660 | (1, 1)  | (2, 1)(3, 1)    | (3, 1)(3, 2)   | $[0, -1 1, 2]$  | K13a1744 |
| 09_23955 | (-1, 1) | (2, 1)(3, 1)    | (3, 1)(4, 1)   | $[0, -1 1, 1]$  | K13a3269 |
| 09_23961 | (0, 1)  | (2, 1)(4, 1)    | (2, 1)(7, 2)   | $[0, -1 1, 0]$  | L13a1655 |
| 09_24149 | (-1, 1) | (2, 1)(3, 1)    | (4, 1)(4, 3)   | $[0, -1 1, 0]$  | L13a3083 |
| 09_24183 | (1, 1)  | (2, 1)(3, 1)    | (3, 2)(8, 5)   | $[0, -1 1, 0]$  | K13a888  |
| 09_24534 | (-1, 1) | (2, 1)(5, 1)    | (3, 1)(3, 1)   | $[0, -1 1, 0]$  | L13a3661 |
| 09_24592 | (-1, 1) | (2, 1)(3, 1)    | (4, 1)(4, 3)   | $[-1, 1 0, 1]$  | L11a255  |
| 09_24886 | (0, 1)  | (2, 1)(2, 1)    | (2, 1)(13, 5)  | $[1, 1  -1, 0]$ | L13a353  |
| 09_24889 | (1, 1)  | (2, 1)(3, 2)    | (2, 1)(10, 3)  | $[0, -1 1, 0]$  | L13a2793 |
| 09_25595 | (-1, 1) | (2, 1)(4, 1)    | (3, 1)(4, 1)   | $[0, -1 1, 0]$  | L13a1946 |
| 09_26604 | (0, 1)  | (2, 1)(3, 1)    | (2, 1)(12, 5)  | $[-1, 1 0, 1]$  | L11a182  |
| 09_26604 | (1, 1)  | (2, 1)(5, 2)    | (2, 1)(7, 5)   | $[-1, 1 0, 1]$  | K11a27   |
| 09_27392 | (-1, 1) | (2, 1)(5, 2)    | (3, 1)(3, 1)   | $[1, 1  -1, 0]$ | L13a3545 |
| 09_27480 | (1, 1)  | (2, 1)(3, 1)    | (3, 1)(3, 1)   | $[2, 1  -1, 0]$ | L13a3645 |
| 09_27737 | (0, 1)  | (2, 1)(4, 1)    | (3, 2)(4, 1)   | $[0, -1 1, 0]$  | L13a1963 |
| 09_28113 | (0, 1)  | (2, 1)(2, 1)    | (4, 1)(5, 2)   | $[1, 1  -1, 0]$ | L13a803  |
| 09_28529 | (-1, 1) | (2, 1)(3, 1)    | (3, 2)(5, 2)   | $[0, -1 1, 1]$  | K13a780  |
| 09_28592 | (0, 1)  | (2, 1)(3, 1)    | (2, 1)(7, 2)   | $[1, 1  -1, 0]$ | K13a1156 |
| 09_29246 | (-1, 1) | (3, 1)(3, 1)    | (3, 2)(5, 3)   | $[0, -1 1, 0]$  | K13a1903 |
| 09_29436 | (0, 1)  | (2, 1)(3, 1)    | (2, 1)(8, 3)   | $[1, 1  -1, 0]$ | L13a1612 |
| 09_29529 | (1, 1)  | (2, 1)(3, 1)    | (2, 1)(13, 5)  | $[-1, 1 0, 1]$  | K11a72   |
| 09_30721 | (0, 1)  | (2, 1)(2, 1)    | (3, 2)(5, 3)   | $[0, -1 1, 0]$  | L11a69   |
| 09_30721 | (1, 1)  | (3, 1)(3, 2)    | (3, 1)(5, 2)   | $[-1, 1 0, 1]$  | K11a157  |
| 09_30790 | (0, 1)  | (2, 1)(5, 3)    | (2, 1)(7, 2)   | $[0, -1 1, 0]$  | K13a9    |
| 09_31165 | (0, 1)  | (2, 1)(4, 1)    | (2, 1)(5, 2)   | $[1, 1  -1, 0]$ | L13a1668 |
| 09_31165 | (1, 1)  | (2, 1)(3, 1)    | (3, 1)(3, 2)   | $[2, 1  -1, 0]$ | K13a912  |
| 09_33526 | (0, 1)  | (2, 1)(5, 2)    | (3, 1)(3, 2)   | $[-1, 1 0, 1]$  | L10a69   |
| 09_33585 | (-1, 1) | (2, 1)(3, 1)    | (4, 3)(5, 2)   | $[-1, 1 0, 1]$  | K11a130  |
| 09_33585 | (0, 1)  | (2, 1)(2, 1)    | (2, 1)(5, 3)   | $[0, -1 1, 1]$  | L11a30   |
| 09_35320 | (-1, 1) | (2, 1)(4, 1)    | (2, 1)(7, 5)   | $[-1, 1 0, 1]$  | L11a149  |
| 09_35549 | (0, 1)  | (2, 1)(3, 2)    | (2, 1)(5, 2)   | $[-1, -1 2, 1]$ | K13a164  |
| 09_35549 | (1, 1)  | (3, 1)(3, 2)    | (3, 2)(5, 3)   | $[0, -1 1, 0]$  | L13a4597 |
| 09_35736 | (0, 1)  | (2, 1)(3, 2)    | (3, 2)(5, 2)   | $[1, 1  -1, 0]$ | L13a2540 |
| 09_35736 | (1, 1)  | (2, 1)(3, 1)    | (3, 2)(5, 3)   | $[1, 1  -1, 0]$ | K13a914  |
| 09_39394 | (0, 1)  | (2, 1)(3, 2)    | (3, 2)(3, 2)   | $[0, -1 1, 0]$  | L11a220  |
| 09_40179 | (0, 1)  | (2, 1)(3, 1)    | (3, 2)(7, 4)   | $[-1, 1 0, 1]$  | K11a298  |

TABLE 11. The complete list of half-integral hyperbolic alternating surgeries along census knots.

| knot              | slope   | branching set     | knot              | slope   | branching set     | knot              | slope   | branching set     |
|-------------------|---------|-------------------|-------------------|---------|-------------------|-------------------|---------|-------------------|
| <i>m</i> 082      | (1, 2)  | <i>K</i> 9a32     | <i>m</i> 144      | (-1, 2) | <i>K</i> 10a97    | <i>m</i> 194      | (1, 2)  | <i>K</i> 10a97    |
| <i>m</i> 198      | (1, 2)  | <i>K</i> 10a118   | <i>m</i> 239      | (-1, 2) | <i>K</i> 9a28     | <i>m</i> 281      | (1, 2)  | <i>K</i> 10a66    |
| <i>s</i> 086      | (-1, 2) | <i>K</i> 11a345   | <i>s</i> 294      | (-1, 2) | <i>K</i> 10a77    | <i>s</i> 301      | (1, 2)  | <i>K</i> 11a146   |
| <i>s</i> 308      | (-1, 2) | <i>K</i> 11a122   | <i>s</i> 336      | (-3, 2) | <i>K</i> 10a85    | <i>s</i> 346      | (1, 2)  | <i>K</i> 11a160   |
| <i>s</i> 367      | (1, 2)  | <i>K</i> 11a168   | <i>s</i> 407      | (-1, 2) | <i>K</i> 11a189   | <i>s</i> 582      | (-1, 2) | <i>K</i> 11a280   |
| <i>s</i> 665      | (1, 2)  | <i>K</i> 11a114   | <i>s</i> 684      | (1, 2)  | <i>K</i> 10a36    | <i>s</i> 800      | (-1, 2) | <i>K</i> 11a209   |
| <i>v</i> 0165     | (1, 2)  | <i>K</i> 12a1063  | <i>v</i> 0330     | (1, 2)  | <i>K</i> 12a1176  | <i>v</i> 0398     | (1, 2)  | <i>K</i> 12a799   |
| <i>v</i> 0407     | (1, 2)  | <i>K</i> 12a1060  | <i>v</i> 0434     | (-1, 2) | <i>K</i> 12a635   | <i>v</i> 0554     | (1, 2)  | <i>K</i> 12a1235  |
| <i>v</i> 0570     | (1, 2)  | <i>K</i> 12a1245  | <i>v</i> 0573     | (-1, 2) | <i>K</i> 12a1239  | <i>v</i> 0707     | (-3, 2) | <i>K</i> 11a256   |
| <i>v</i> 0740     | (1, 2)  | <i>K</i> 12a781   | <i>v</i> 0759     | (-1, 2) | <i>K</i> 12a646   | <i>v</i> 0765     | (-1, 2) | <i>K</i> 12a751   |
| <i>v</i> 0939     | (-1, 2) | <i>K</i> 11a255   | <i>v</i> 0945     | (1, 2)  | <i>K</i> 12a614   | <i>v</i> 1077     | (1, 2)  | <i>K</i> 12a287   |
| <i>v</i> 1109     | (-1, 2) | <i>K</i> 12a470   | <i>v</i> 1392     | (-3, 2) | <i>K</i> 11a282   | <i>v</i> 1547     | (-3, 2) | <i>K</i> 11a290   |
| <i>v</i> 1620     | (1, 2)  | <i>K</i> 12a1169  | <i>v</i> 1690     | (-3, 2) | <i>K</i> 11a101   | <i>v</i> 1709     | (-1, 2) | <i>K</i> 11a773   |
| <i>v</i> 1716     | (3, 2)  | <i>K</i> 11a300   | <i>v</i> 1718     | (-1, 2) | <i>K</i> 12a1182  | <i>v</i> 1728     | (3, 2)  | <i>K</i> 11a272   |
| <i>v</i> 1810     | (-1, 2) | <i>K</i> 12a308   | <i>v</i> 1832     | (1, 2)  | <i>K</i> 11a136   | <i>v</i> 1839     | (-1, 2) | <i>K</i> 12a261   |
| <i>v</i> 1921     | (-1, 2) | <i>K</i> 12a1048  | <i>v</i> 1980     | (-1, 2) | <i>K</i> 10a88    | <i>v</i> 1986     | (-1, 2) | <i>K</i> 12a770   |
| <i>v</i> 2024     | (1, 2)  | <i>K</i> 12a766   | <i>v</i> 2090     | (-1, 2) | <i>K</i> 12a310   | <i>v</i> 2215     | (1, 2)  | <i>K</i> 11a138   |
| <i>v</i> 2325     | (-1, 2) | <i>K</i> 12a608   | <i>v</i> 2759     | (1, 2)  | <i>K</i> 12a1169  | <i>v</i> 2930     | (-1, 2) | <i>K</i> 12a1258  |
| <i>v</i> 3354     | (1, 2)  | <i>K</i> 12a604   | <i>v</i> 00324    | (-1, 2) | <i>K</i> 13a4578  | <i>v</i> 00729    | (-1, 2) | <i>K</i> 13a3026  |
| <i>v</i> 00787    | (1, 2)  | <i>K</i> 13a2738  | <i>v</i> 00826    | (1, 2)  | <i>K</i> 13a2435  | <i>v</i> 00855    | (-1, 2) | <i>K</i> 13a1915  |
| <i>v</i> 01033    | (1, 2)  | <i>K</i> 13a4277  | <i>v</i> 01037    | (-1, 2) | <i>K</i> 13a4271  | <i>v</i> 01125    | (1, 2)  | <i>K</i> 13a3911  |
| <i>v</i> 01268    | (1, 2)  | <i>K</i> 13a1896  | <i>v</i> 01318    | (1, 2)  | <i>K</i> 12a807   | <i>v</i> 01368    | (1, 2)  | <i>K</i> 12a358   |
| <i>v</i> 01422    | (-3, 2) | <i>K</i> 12a858   | <i>v</i> 01440    | (1, 2)  | <i>K</i> 13a2587  | <i>v</i> 01636    | (1, 2)  | <i>K</i> 13a3939  |
| <i>v</i> 01690    | (1, 2)  | <i>K</i> 13a2743  | <i>v</i> 01757    | (-1, 2) | <i>K</i> 13a2915  | <i>v</i> 01834    | (-1, 2) | <i>K</i> 13a2739  |
| <i>v</i> 01863    | (1, 2)  | <i>K</i> 13a3748  | <i>v</i> 02099    | (-3, 2) | <i>K</i> 12a821   | <i>v</i> 02104    | (-1, 2) | <i>K</i> 12a670   |
| <i>v</i> 02238    | (-1, 2) | <i>K</i> 13a2380  | <i>v</i> 02378    | (-1, 2) | <i>K</i> 13a1806  | <i>v</i> 02398    | (-1, 2) | <i>K</i> 13a1983  |
| <i>v</i> 02404    | (-1, 2) | <i>K</i> 12a415   | <i>v</i> 02470    | (1, 2)  | <i>K</i> 13a2082  | <i>v</i> 02537    | (-1, 2) | <i>K</i> 13a2460  |
| <i>v</i> 02567    | (-1, 2) | <i>K</i> 13a2737  | <i>v</i> 02639    | (1, 2)  | <i>K</i> 13a794   | <i>v</i> 03607    | (1, 2)  | <i>K</i> 13a1605  |
| <i>v</i> 03713    | (-3, 2) | <i>K</i> 12a360   | <i>v</i> 03781    | (1, 2)  | <i>K</i> 13a3991  | <i>v</i> 03864    | (3, 2)  | <i>K</i> 12a202   |
| <i>v</i> 03956    | (-3, 2) | <i>K</i> 12a919   | <i>v</i> 03979    | (-1, 2) | <i>K</i> 12a865   | <i>v</i> 04003    | (-3, 2) | <i>K</i> 12a455   |
| <i>v</i> 04019    | (-1, 2) | <i>K</i> 13a4402  | <i>v</i> 04102    | (3, 2)  | <i>K</i> 12a407   | <i>v</i> 04180    | (-1, 2) | <i>K</i> 13a2187  |
| <i>v</i> 04244    | (2, 1)  | <i>K</i> 13a1016  | <i>v</i> 04382    | (1, 2)  | <i>K</i> 13a2731  | <i>v</i> 04721    | (2, 1)  | <i>K</i> 13a4582  |
| <i>v</i> 05118    | (-1, 2) | <i>K</i> 13a1626  | <i>v</i> 05390    | (-3, 2) | <i>K</i> 12a1268  | <i>v</i> 05425    | (1, 2)  | <i>K</i> 12a656   |
| <i>v</i> 05538    | (-1, 2) | <i>K</i> 12a559   | <i>v</i> 05564    | (-1, 2) | <i>K</i> 13a2522  | <i>v</i> 05658    | (2, 1)  | <i>K</i> 12a631   |
| <i>v</i> 05674    | (-1, 2) | <i>K</i> 13a1655  | <i>v</i> 05695    | (-1, 2) | <i>K</i> 13a2869  | <i>v</i> 06001    | (-2, 1) | <i>K</i> 13a2963  |
| <i>v</i> 06440    | (-1, 2) | <i>K</i> 13a2202  | <i>v</i> 06463    | (1, 2)  | <i>K</i> 13a1008  | <i>v</i> 06525    | (1, 2)  | <i>K</i> 12a695   |
| <i>v</i> 06570    | (-1, 2) | <i>K</i> 13a2495  | <i>v</i> 06605    | (1, 2)  | <i>K</i> 13a885   | <i>v</i> 07348    | (-1, 2) | <i>K</i> 11a233   |
| <i>v</i> 08111    | (-1, 2) | <i>K</i> 11a283   | <i>v</i> 08201    | (1, 2)  | <i>K</i> 11a233   | <i>v</i> 08267    | (1, 2)  | <i>K</i> 12a209   |
| <i>v</i> 08403    | (-1, 2) | <i>K</i> 12a346   | <i>v</i> 09016    | (-1, 2) | <i>K</i> 12a426   | <i>v</i> 09267    | (1, 2)  | <i>K</i> 13a1011  |
| <i>v</i> 09313    | (1, 2)  | <i>K</i> 13a1035  | <i>v</i> 09455    | (-1, 2) | <i>K</i> 13a1649  | <i>v</i> 09580    | (-1, 2) | <i>K</i> 12a637   |
| <i>v</i> 09704    | (-1, 2) | <i>K</i> 13a1282  | <i>v</i> 09852    | (1, 2)  | <i>K</i> 11a289   | <i>v</i> 09954    | (-1, 2) | <i>K</i> 11a351   |
| <i>v</i> 10230    | (1, 2)  | <i>K</i> 11a289   | <i>v</i> 10462    | (-1, 2) | <i>K</i> 12a588   | <i>v</i> 10643    | (1, 2)  | <i>K</i> 13a1714  |
| <i>v</i> 10681    | (-1, 2) | <i>K</i> 13a1574  | <i>v</i> 10985    | (-1, 2) | <i>K</i> 13a1963  | <i>v</i> 11852    | (1, 2)  | <i>K</i> 11a326   |
| <i>v</i> 09_00644 | (-1, 2) | <i>K</i> 14a16783 | <i>v</i> 09_01436 | (1, 2)  | <i>K</i> 14a17856 | <i>v</i> 09_01496 | (-1, 2) | <i>K</i> 14a15197 |
| <i>v</i> 09_01584 | (-1, 2) | <i>K</i> 14a16756 | <i>v</i> 09_01621 | (1, 2)  | <i>K</i> 14a16609 | <i>v</i> 09_01953 | (1, 2)  | <i>K</i> 14a18519 |
| <i>v</i> 09_01955 | (1, 2)  | <i>K</i> 14a18499 | <i>v</i> 09_02255 | (1, 2)  | <i>K</i> 14a7592  | <i>v</i> 09_02350 | (1, 2)  | <i>K</i> 14a7103  |
| <i>v</i> 09_02655 | (-1, 2) | <i>K</i> 13a1443  | <i>v</i> 09_02696 | (-1, 2) | <i>K</i> 13a761   | <i>v</i> 09_02772 | (-1, 2) | <i>K</i> 14a18477 |
| <i>v</i> 09_02786 | (-3, 2) | <i>K</i> 13a3307  | <i>v</i> 09_02794 | (1, 2)  | <i>K</i> 14a12509 | <i>v</i> 09_03032 | (-1, 2) | <i>K</i> 14a11620 |
| <i>v</i> 09_03108 | (-1, 2) | <i>K</i> 14a19430 | <i>v</i> 09_03133 | (1, 2)  | <i>K</i> 14a16622 | <i>v</i> 09_03162 | (1, 2)  | <i>K</i> 14a10625 |
| <i>v</i> 09_03188 | (1, 2)  | <i>K</i> 14a10099 | <i>v</i> 09_03313 | (1, 2)  | <i>K</i> 14a10266 | <i>v</i> 09_03586 | (-1, 2) | <i>K</i> 14a19105 |
| <i>v</i> 09_03622 | (-1, 2) | <i>K</i> 14a17463 | <i>v</i> 09_03802 | (-1, 2) | <i>K</i> 14a19111 | <i>v</i> 09_03833 | (-1, 2) | <i>K</i> 14a10696 |
| <i>v</i> 09_04106 | (1, 2)  | <i>K</i> 14a12339 | <i>v</i> 09_04205 | (1, 2)  | <i>K</i> 14a7694  | <i>v</i> 09_04245 | (-1, 2) | <i>K</i> 14a10812 |
| <i>v</i> 09_04269 | (-3, 2) | <i>K</i> 13a3201  | <i>v</i> 09_04438 | (-1, 2) | <i>K</i> 14a8243  | <i>v</i> 09_05021 | (-1, 2) | <i>K</i> 14a11003 |
| <i>v</i> 09_05177 | (-1, 2) | <i>K</i> 14a11048 | <i>v</i> 09_05229 | (-1, 2) | <i>K</i> 14a12627 | <i>v</i> 09_05357 | (-1, 2) | <i>K</i> 14a11003 |
| <i>v</i> 09_05426 | (-1, 2) | <i>K</i> 14a10190 | <i>v</i> 09_05483 | (-1, 2) | <i>K</i> 14a9562  | <i>v</i> 09_05562 | (-1, 2) | <i>K</i> 14a10897 |
| <i>v</i> 09_05618 | (-1, 2) | <i>K</i> 14a9163  | <i>v</i> 09_05860 | (-1, 2) | <i>K</i> 14a8262  | <i>v</i> 09_05970 | (-1, 2) | <i>K</i> 14a6783  |
| <i>v</i> 09_06060 | (1, 2)  | <i>K</i> 13a1328  | <i>v</i> 09_06128 | (-1, 2) | <i>K</i> 14a7129  | <i>v</i> 09_06154 | (1, 2)  | <i>K</i> 13a1509  |
| <i>v</i> 09_06248 | (-1, 2) | <i>K</i> 14a2949  | <i>v</i> 09_06301 | (-1, 2) | <i>K</i> 14a6547  | <i>v</i> 09_07790 | (-1, 2) | <i>K</i> 14a17873 |
| <i>v</i> 09_07893 | (-1, 2) | <i>K</i> 13a3150  | <i>v</i> 09_07945 | (-1, 2) | <i>K</i> 13a1843  | <i>v</i> 09_08006 | (-1, 2) | <i>K</i> 14a11327 |
| <i>v</i> 09_08224 | (3, 2)  | <i>K</i> 13a3634  | <i>v</i> 09_08302 | (3, 2)  | <i>K</i> 13a3547  | <i>v</i> 09_08477 | (1, 2)  | <i>K</i> 14a17811 |
| <i>v</i> 09_08647 | (2, 1)  | <i>K</i> 14a8937  | <i>v</i> 09_08765 | (-3, 2) | <i>K</i> 13a3671  | <i>v</i> 09_08771 | (2, 1)  | <i>K</i> 14a6761  |
| <i>v</i> 09_08828 | (-1, 2) | <i>K</i> 14a16699 | <i>v</i> 09_08831 | (-3, 2) | <i>K</i> 13a3803  | <i>v</i> 09_08875 | (-1, 2) | <i>K</i> 14a11069 |
| <i>v</i> 09_09213 | (1, 2)  | <i>K</i> 14a7691  | <i>v</i> 09_09465 | (-1, 2) | <i>K</i> 14a7568  | <i>v</i> 09_09808 | (-1, 2) | <i>K</i> 14a10354 |
| <i>v</i> 09_11248 | (2, 1)  | <i>K</i> 14a17871 | <i>v</i> 09_11570 | (1, 2)  | <i>K</i> 14a16575 | <i>v</i> 09_11685 | (3, 2)  | <i>K</i> 13a4143  |
| <i>v</i> 09_11795 | (-3, 2) | <i>K</i> 13a4228  | <i>v</i> 09_11845 | (-3, 2) | <i>K</i> 13a3487  | <i>v</i> 09_11999 | (2, 1)  | <i>K</i> 14a11475 |
| <i>v</i> 09_12412 | (3, 2)  | <i>K</i> 13a2257  | <i>v</i> 09_12459 | (-2, 1) | <i>K</i> 13a2345  | <i>v</i> 09_12519 | (-1, 2) | <i>K</i> 13a2254  |
| <i>v</i> 09_12693 | (-1, 2) | <i>K</i> 14a19195 | <i>v</i> 09_12757 | (-1, 2) | <i>K</i> 14a10775 | <i>v</i> 09_12873 | (-1, 2) | <i>K</i> 14a5793  |
| <i>v</i> 09_12892 | (-3, 2) | <i>K</i> 13a4426  | <i>v</i> 09_12919 | (-3, 2) | <i>K</i> 13a3486  | <i>v</i> 09_12971 | (-1, 2) | <i>K</i> 13a2347  |
| <i>v</i> 09_13052 | (-2, 1) | <i>K</i> 14a12642 | <i>v</i> 09_13125 | (2, 1)  | <i>K</i> 13a1834  | <i>v</i> 09_13182 | (-3, 2) | <i>K</i> 13a4754  |
| <i>v</i> 09_13188 | (-1, 2) | <i>K</i> 14a12639 | <i>v</i> 09_13400 | (-1, 2) | <i>K</i> 14a17456 | <i>v</i> 09_13403 | (-3, 2) | <i>K</i> 13a2904  |
| <i>v</i> 09_13433 | (1, 2)  | <i>K</i> 13a1734  | <i>v</i> 09_13537 | (-3, 2) | <i>K</i> 13a1664  | <i>v</i> 09_13604 | (-1, 2) | <i>K</i> 14a12420 |
| <i>v</i> 09_13639 | (1, 2)  | <i>K</i> 13a4371  | <i>v</i> 09_13649 | (3, 2)  | <i>K</i> 13a2011  | <i>v</i> 09_13666 | (2, 1)  | <i>K</i> 14a19167 |
| <i>v</i> 09_13720 | (1, 2)  | <i>K</i> 14a7490  | <i>v</i> 09_13952 | (1, 2)  | <i>K</i> 14a10121 | <i>v</i> 09_14079 | (-1, 2) | <i>K</i> 14a4414  |

TABLE 12. Table 11 continued.

| knot     | slope   | branching set | knot     | slope   | branching set | knot     | slope   | branching set |
|----------|---------|---------------|----------|---------|---------------|----------|---------|---------------|
| o9_14364 | (-3, 2) | K13a3952      | o9_14376 | (1, 2)  | K14a6097      | o9_14495 | (-3, 2) | K13a2218      |
| o9_14599 | (-1, 2) | K14a12304     | o9_14716 | (-1, 2) | K14a18651     | o9_14831 | (-1, 2) | K12a864       |
| o9_14974 | (1, 2)  | K14a11401     | o9_15506 | (3, 2)  | K13a1178      | o9_15633 | (1, 2)  | K13a2658      |
| o9_15997 | (-1, 2) | K14a10710     | o9_16065 | (-1, 2) | K14a7006      | o9_16141 | (-1, 2) | K14a5782      |
| o9_16157 | (-1, 2) | K14a5900      | o9_16181 | (1, 2)  | K14a8736      | o9_16319 | (-1, 2) | K14a4566      |
| o9_16356 | (1, 2)  | K14a18894     | o9_16527 | (1, 2)  | K14a18817     | o9_16642 | (-1, 2) | K14a3526      |
| o9_16748 | (-1, 2) | K13a1775      | o9_16920 | (-1, 2) | K12a631       | o9_17450 | (-3, 2) | K13a2563      |
| o9_18007 | (-1, 2) | K13a2363      | o9_18209 | (1, 2)  | K14a10774     | o9_18633 | (-3, 2) | K13a3082      |
| o9_18813 | (1, 2)  | K12a696       | o9_19130 | (1, 2)  | K12a857       | o9_20219 | (-1, 2) | K13a3718      |
| o9_21893 | (-2, 1) | K12a1199      | o9_21918 | (-1, 2) | K12a1228      | o9_22129 | (-1, 2) | K14a19388     |
| o9_22477 | (-1, 2) | K12a1231      | o9_22607 | (1, 2)  | K14a19195     | o9_22663 | (-1, 2) | K12a316       |
| o9_22698 | (1, 2)  | K13a1395      | o9_22925 | (-1, 2) | K12a309       | o9_23023 | (1, 2)  | K13a713       |
| o9_23263 | (1, 2)  | K14a17804     | o9_23660 | (1, 2)  | K14a11215     | o9_23955 | (-1, 2) | K14a19194     |
| o9_23961 | (1, 2)  | K14a12666     | o9_23977 | (1, 2)  | K13a3677      | o9_24149 | (-1, 2) | K14a19179     |
| o9_24183 | (2, 1)  | K14a3347      | o9_24534 | (-2, 1) | K14a18856     | o9_24592 | (-1, 2) | K12a1271      |
| o9_24886 | (-1, 2) | K14a7920      | o9_24889 | (1, 2)  | K14a12495     | o9_25595 | (-1, 2) | K14a19452     |
| o9_26604 | (1, 2)  | K12a793       | o9_26791 | (-1, 2) | K13a2340      | o9_27155 | (1, 2)  | K13a1194      |
| o9_27261 | (-1, 2) | K13a2311      | o9_27392 | (-1, 2) | K14a3943      | o9_27480 | (1, 2)  | K14a7535      |
| o9_27737 | (1, 2)  | K14a12587     | o9_28113 | (1, 2)  | K14a11153     | o9_28153 | (1, 2)  | K13a1374      |
| o9_28529 | (-2, 1) | K14a3324      | o9_28592 | (-1, 2) | K14a7952      | o9_28746 | (-1, 2) | K13a2505      |
| o9_28810 | (1, 2)  | K13a1132      | o9_29246 | (-1, 2) | K14a5848      | o9_29436 | (1, 2)  | K14a10851     |
| o9_29529 | (1, 2)  | K12a359       | o9_30375 | (1, 2)  | K13a1092      | o9_30721 | (1, 2)  | K12a467       |
| o9_30790 | (1, 2)  | K14a7870      | o9_31165 | (1, 2)  | K14a10885     | o9_32257 | (1, 2)  | K12a993       |
| o9_33526 | (-1, 2) | K11a287       | o9_33585 | (-1, 2) | K12a340       | o9_34403 | (-1, 2) | K12a1198      |
| o9_35320 | (-1, 2) | K12a1217      | o9_35549 | (1, 2)  | K14a3551      | o9_35682 | (1, 2)  | K12a1081      |
| o9_35736 | (1, 2)  | K14a6098      | o9_35772 | (-1, 2) | K12a966       | o9_37941 | (-1, 2) | K12a1005      |
| o9_39394 | (1, 2)  | K12a765       |          |         |               |          |         |               |

TABLE 13. The complete list of all exceptional half-integer alternating surgeries. All fillings are graph manifolds obtained by gluing together two Seifert fibered spaces with base  $D^2$  and with 2 exceptional fibers. The columns titled *filled manifold* gives Regina's notation for the graph manifold.

| knot   | slope   | filled manifold |                |                | branching set |
|--------|---------|-----------------|----------------|----------------|---------------|
| m016   | (-1, 2) | (2, 1)(3, 1)    | (2, 1)(3, 2)   | $[-1, 1 0, 1]$ | K8a14         |
| m071   | (-1, 2) | (2, 1)(3, 1)    | (2, 1)(5, 4)   | $[-1, 1 0, 1]$ | K10a83        |
| m103   | (-1, 2) | (2, 1)(3, 1)    | (2, 1)(7, 5)   | $[-1, 1 0, 1]$ | K10a50        |
| m118   | (-1, 2) | (2, 1)(3, 1)    | (2, 1)(5, 3)   | $[-1, 1 0, 1]$ | K9a11         |
| m240   | (-2, 1) | (2, 1)(3, 1)    | (3, 1)(4, 3)   | $[-1, 1 0, 1]$ | K10a106       |
| m270   | (2, 1)  | (2, 1)(3, 1)    | (3, 2)(5, 2)   | $[-1, 1 0, 1]$ | K10a47        |
| m276   | (2, 1)  | (2, 1)(5, 2)    | (2, 1)(5, 3)   | $[-1, 1 0, 1]$ | K10a11        |
| s042   | (1, 2)  | (2, 1)(3, 1)    | (2, 1)(9, 7)   | $[-1, 1 0, 1]$ | K11a167       |
| s068   | (-1, 2) | (2, 1)(3, 1)    | (2, 1)(11, 8)  | $[-1, 1 0, 1]$ | K11a80        |
| s104   | (-1, 2) | (2, 1)(3, 1)    | (2, 1)(11, 7)  | $[-1, 1 0, 1]$ | K11a264       |
| s114   | (-1, 2) | (2, 1)(3, 1)    | (2, 1)(13, 8)  | $[-1, 1 0, 1]$ | K11a71        |
| s344   | (2, 1)  | (2, 1)(3, 1)    | (3, 1)(7, 5)   | $[-1, 1 0, 1]$ | K11a149       |
| s369   | (-2, 1) | (2, 1)(5, 2)    | (2, 1)(7, 4)   | $[-1, 1 0, 1]$ | K11a69        |
| s769   | (1, 1)  | (2, 1)(5, 2)    | (3, 2)(5, 2)   | $[-1, 1 0, 1]$ | K11a70        |
| v0082  | (1, 2)  | (2, 1)(3, 1)    | (2, 1)(13, 10) | $[-1, 1 0, 1]$ | K12a851       |
| v0114  | (1, 2)  | (2, 1)(3, 1)    | (2, 1)(15, 11) | $[-1, 1 0, 1]$ | K12a849       |
| v0220  | (1, 2)  | (2, 1)(3, 1)    | (2, 1)(19, 12) | $[-1, 1 0, 1]$ | K12a282       |
| v0223  | (1, 2)  | (2, 1)(3, 1)    | (2, 1)(21, 13) | $[-1, 1 0, 1]$ | K12a214       |
| v0424  | (2, 1)  | (2, 1)(3, 1)    | (3, 2)(9, 4)   | $[-1, 1 0, 1]$ | K12a944       |
| v0497  | (2, 1)  | (2, 1)(3, 1)    | (3, 2)(12, 5)  | $[-1, 1 0, 1]$ | K12a509       |
| v0709  | (2, 1)  | (2, 1)(3, 1)    | (4, 1)(5, 4)   | $[-1, 1 0, 1]$ | K12a1011      |
| v0715  | (-2, 1) | (2, 1)(5, 2)    | (2, 1)(11, 7)  | $[-1, 1 0, 1]$ | K12a138       |
| v0741  | (2, 1)  | (2, 1)(5, 2)    | (2, 1)(13, 8)  | $[-1, 1 0, 1]$ | K12a191       |
| v0847  | (-2, 1) | (2, 1)(3, 1)    | (4, 3)(7, 2)   | $[-1, 1 0, 1]$ | K12a606       |
| v0912  | (2, 1)  | (2, 1)(7, 3)    | (2, 1)(7, 4)   | $[-1, 1 0, 1]$ | K12a1008      |
| v1300  | (-1, 1) | (2, 1)(5, 1)    | (3, 1)(4, 3)   | $[-1, 1 0, 1]$ | K12a1219      |
| v1628  | (-1, 1) | (2, 1)(7, 2)    | (3, 1)(4, 3)   | $[-1, 1 0, 1]$ | K12a290       |
| v1940  | (-1, 1) | (2, 1)(5, 2)    | (3, 1)(7, 5)   | $[-1, 1 0, 1]$ | K12a73        |
| v1966  | (-1, 1) | (2, 1)(5, 2)    | (3, 2)(8, 3)   | $[-1, 1 0, 1]$ | K12a184       |
| t00110 | (1, 2)  | (2, 1)(3, 1)    | (2, 1)(17, 13) | $[-1, 1 0, 1]$ | K13a3353      |
| t00146 | (-1, 2) | (2, 1)(3, 1)    | (2, 1)(19, 14) | $[-1, 1 0, 1]$ | K13a3362      |
| t00423 | (-1, 2) | (2, 1)(3, 1)    | (2, 1)(27, 17) | $[-1, 1 0, 1]$ | K13a3384      |
| t00434 | (1, 2)  | (2, 1)(3, 1)    | (2, 1)(29, 18) | $[-1, 1 0, 1]$ | K13a3361      |
| t00873 | (2, 1)  | (2, 1)(3, 1)    | (3, 2)(16, 7)  | $[-1, 1 0, 1]$ | K13a2071      |
| t00932 | (-2, 1) | (2, 1)(3, 1)    | (3, 2)(19, 8)  | $[-1, 1 0, 1]$ | K13a1907      |
| t01216 | (2, 1)  | (2, 1)(3, 1)    | (3, 1)(15, 11) | $[-1, 1 0, 1]$ | K13a3907      |

TABLE 14. Table 13 continued.

| knot       | slope   | filled manifold |                | branching set  |             |
|------------|---------|-----------------|----------------|----------------|-------------|
| $t01292$   | (2, 1)  | (2, 1)(3, 1)    | (3, 1)(18, 13) | $[-1, 1 0, 1]$ | $K13a1805$  |
| $t01409$   | (2, 1)  | (2, 1)(5, 2)    | (2, 1)(19, 12) | $[-1, 1 0, 1]$ | $K13a615$   |
| $t01424$   | (-2, 1) | (2, 1)(5, 2)    | (2, 1)(21, 13) | $[-1, 1 0, 1]$ | $K13a439$   |
| $t01598$   | (-2, 1) | (2, 1)(5, 2)    | (2, 1)(17, 10) | $[-1, 1 0, 1]$ | $K13a680$   |
| $t01646$   | (-2, 1) | (2, 1)(5, 2)    | (2, 1)(19, 11) | $[-1, 1 0, 1]$ | $K13a442$   |
| $t01850$   | (2, 1)  | (2, 1)(3, 1)    | (4, 1)(9, 7)   | $[-1, 1 0, 1]$ | $K13a2519$  |
| $t01949$   | (2, 1)  | (2, 1)(7, 3)    | (2, 1)(9, 5)   | $[-1, 1 0, 1]$ | $K13a3826$  |
| $t03566$   | (1, 1)  | (2, 1)(9, 2)    | (3, 1)(4, 3)   | $[-1, 1 0, 1]$ | $K13a1285$  |
| $t03709$   | (-1, 1) | (2, 1)(11, 3)   | (3, 1)(4, 3)   | $[-1, 1 0, 1]$ | $K13a806$   |
| $t04228$   | (1, 1)  | (2, 1)(5, 2)    | (3, 1)(10, 7)  | $[-1, 1 0, 1]$ | $K13a221$   |
| $t05239$   | (-1, 1) | (2, 1)(11, 4)   | (3, 2)(5, 2)   | $[-1, 1 0, 1]$ | $K13a1364$  |
| $t05426$   | (-1, 1) | (2, 1)(13, 5)   | (3, 2)(5, 2)   | $[-1, 1 0, 1]$ | $K13a821$   |
| $t05578$   | (1, 1)  | (2, 1)(7, 3)    | (3, 2)(8, 3)   | $[-1, 1 0, 1]$ | $K13a715$   |
| $t05663$   | (-1, 1) | (2, 1)(5, 2)    | (4, 3)(7, 2)   | $[-1, 1 0, 1]$ | $K13a607$   |
| $o9.00133$ | (-1, 2) | (2, 1)(3, 1)    | (2, 1)(21, 16) | $[-1, 1 0, 1]$ | $K14a13432$ |
| $o9.00168$ | (1, 2)  | (2, 1)(3, 1)    | (2, 1)(23, 17) | $[-1, 1 0, 1]$ | $K14a13417$ |
| $o9.00797$ | (-1, 2) | (2, 1)(3, 1)    | (2, 1)(35, 22) | $[-1, 1 0, 1]$ | $K14a13298$ |
| $o9.00815$ | (-1, 2) | (2, 1)(3, 1)    | (2, 1)(37, 23) | $[-1, 1 0, 1]$ | $K14a13403$ |
| $o9.01680$ | (2, 1)  | (2, 1)(3, 1)    | (3, 2)(23, 10) | $[-1, 1 0, 1]$ | $K14a14297$ |
| $o9.01765$ | (-2, 1) | (2, 1)(3, 1)    | (3, 2)(26, 11) | $[-1, 1 0, 1]$ | $K14a13889$ |
| $o9.02340$ | (-2, 1) | (2, 1)(3, 1)    | (3, 1)(26, 19) | $[-1, 1 0, 1]$ | $K14a7439$  |
| $o9.02386$ | (-2, 1) | (2, 1)(3, 1)    | (3, 1)(29, 21) | $[-1, 1 0, 1]$ | $K14a6987$  |
| $o9.02706$ | (-2, 1) | (2, 1)(5, 2)    | (2, 1)(27, 17) | $[-1, 1 0, 1]$ | $K14a2247$  |
| $o9.02735$ | (2, 1)  | (2, 1)(5, 2)    | (2, 1)(29, 18) | $[-1, 1 0, 1]$ | $K14a2615$  |
| $o9.03118$ | (-2, 1) | (2, 1)(5, 2)    | (2, 1)(29, 17) | $[-1, 1 0, 1]$ | $K14a1536$  |
| $o9.03149$ | (2, 1)  | (2, 1)(5, 2)    | (2, 1)(31, 18) | $[-1, 1 0, 1]$ | $K14a2613$  |
| $o9.03288$ | (2, 1)  | (2, 1)(3, 1)    | (4, 3)(13, 4)  | $[-1, 1 0, 1]$ | $K14a14831$ |
| $o9.03412$ | (2, 1)  | (2, 1)(3, 1)    | (4, 3)(17, 5)  | $[-1, 1 0, 1]$ | $K14a10105$ |
| $o9.03526$ | (-2, 1) | (2, 1)(3, 1)    | (5, 1)(6, 5)   | $[-1, 1 0, 1]$ | $K14a16396$ |
| $o9_03932$ | (2, 1)  | (2, 1)(3, 1)    | (5, 4)(9, 2)   | $[-1, 1 0, 1]$ | $K14a11193$ |
| $o9.04313$ | (2, 1)  | (2, 1)(7, 3)    | (2, 1)(17, 10) | $[-1, 1 0, 1]$ | $K14a14819$ |
| $o9.04431$ | (2, 1)  | (2, 1)(7, 3)    | (2, 1)(19, 11) | $[-1, 1 0, 1]$ | $K14a5832$  |
| $o9.04435$ | (2, 1)  | (2, 1)(9, 4)    | (2, 1)(9, 5)   | $[-1, 1 0, 1]$ | $K14a14873$ |
| $o9.07943$ | (-1, 1) | (2, 1)(13, 3)   | (3, 1)(4, 3)   | $[-1, 1 0, 1]$ | $K14a18265$ |
| $o9.08042$ | (1, 1)  | (2, 1)(15, 4)   | (3, 1)(4, 3)   | $[-1, 1 0, 1]$ | $K14a14990$ |
| $o9.08776$ | (1, 1)  | (2, 1)(5, 2)    | (3, 2)(18, 7)  | $[-1, 1 0, 1]$ | $K14a2564$  |
| $o9.08852$ | (1, 1)  | (2, 1)(5, 2)    | (3, 2)(21, 8)  | $[-1, 1 0, 1]$ | $K14a2653$  |
| $o9.10696$ | (-1, 1) | (2, 1)(5, 1)    | (4, 1)(5, 4)   | $[-1, 1 0, 1]$ | $K14a18376$ |
| $o9.11467$ | (-1, 1) | (2, 1)(19, 7)   | (3, 2)(5, 2)   | $[-1, 1 0, 1]$ | $K14a3771$  |
| $o9.11560$ | (-1, 1) | (2, 1)(21, 8)   | (3, 2)(5, 2)   | $[-1, 1 0, 1]$ | $K14a3245$  |
| $o9.12144$ | (1, 1)  | (2, 1)(7, 3)    | (3, 1)(10, 7)  | $[-1, 1 0, 1]$ | $K14a17264$ |
| $o9.12230$ | (-1, 1) | (2, 1)(7, 3)    | (3, 2)(11, 4)  | $[-1, 1 0, 1]$ | $K14a15078$ |
| $o9.12736$ | (1, 1)  | (2, 1)(5, 2)    | (4, 1)(9, 7)   | $[-1, 1 0, 1]$ | $K14a771$   |
| $o9.13056$ | (-1, 1) | (2, 1)(5, 2)    | (4, 3)(11, 3)  | $[-1, 1 0, 1]$ | $K14a1548$  |
| $o9.13508$ | (1, 1)  | (2, 1)(11, 4)   | (3, 1)(7, 5)   | $[-1, 1 0, 1]$ | $K14a5545$  |
| $o9.14018$ | (1, 1)  | (2, 1)(13, 5)   | (3, 1)(7, 5)   | $[-1, 1 0, 1]$ | $K14a3045$  |
| $o9.14136$ | (-1, 1) | (2, 1)(7, 2)    | (4, 1)(5, 4)   | $[-1, 1 0, 1]$ | $K14a5717$  |
